# Supplementary material for: From Heteropolymer Stiffness Distributions to Effective Homopolymers: A Conformational Analysis of Intrinsically Disordered Proteins
Source: arXiv:2504.11027 source file (2025-11-03)
Supplement: Supplementary file 1 [file SI.pdf]

## Supplementary Material: From Heteropolymer Stiffness Distributions to Effective Homopolymers: A Conformational Analysis of Intrinsically Disordered Proteins

Yannick Witzky,<sup>1</sup> Friederike Schmid,<sup>1, a)</sup> and Arash Nikoubashman<sup>2, 3, 4, b)</sup>

<sup>1)</sup>*Institute of Physics, Johannes Gutenberg University Mainz, Staudingerweg 7-9, 55128 Mainz, Germany*

<sup>2)</sup>*Leibniz-Institut für Polymerforschung Dresden e.V., Hohe Straße 6, 01069 Dresden, Germany*

<sup>3)</sup>*Institut für Theoretische Physik, Technische Universität Dresden, 01069 Dresden, Germany*

<sup>4)</sup>*Cluster of Excellence Physics of Life, Technische Universität Dresden, 01062 Dresden, Germany*

---

<sup>a)</sup>Electronic mail: [friederike.schmid@uni-mainz.de](mailto:friederike.schmid@uni-mainz.de)

<sup>b)</sup>Electronic mail: [anikouba@ipfdd.de](mailto:anikouba@ipfdd.de)

# I. THEORY FOR EFFECTIVE PERSISTENCE LENGTH IN HETEROGENEOUS IDEAL CHAINS

## A. Model assumptions and goal

We consider ideal chains of length  $N$  with the angular potential

$$U_{\text{bend}} = k_{\text{B}}T \sum_i \kappa_i (1 - \mathbf{u}_i \cdot \mathbf{u}_{i+1}) = k_{\text{B}}T \sum_i \kappa_i [1 - \cos(\theta)] \quad (\text{S1})$$

where  $\mathbf{u}_i$  are unit vectors pointing in the direction of the bonds with length  $b$ . The angle potential parameters  $\kappa_i$  are Gaussian distributed with mean  $\kappa_0$  and variance  $\sigma_{\kappa}^2$ , i.e., the distribution is

$$P(\kappa_i) = \frac{1}{\sqrt{2\pi}\sigma} \exp \left[ -\frac{(\kappa_i - \kappa_0)^2}{2\sigma_{\kappa}^2} \right]. \quad (\text{S2})$$

Moreover, we assume that the different angle potential parameters are uncorrelated,  $\langle \kappa_i \kappa_j \rangle - \kappa_0^2 = \delta_{ij} \sigma^2$  (this assumption can be dropped if necessary).

The local persistence length  $\ell_{\text{p}}(\kappa_i)$  is defined via the relation<sup>1</sup>

$$\langle \mathbf{u}_i \cdot \mathbf{u}_{i+1} \rangle = \exp [-\ell_{\text{p}}(\kappa_i)/b], \quad (\text{S3})$$

where  $\langle \cdot \rangle$  denotes the thermal average. Since the model only includes bending potentials, it can easily be evaluated, resulting in

$$\ell_{\text{p}}(\kappa_i) = -b / \ln [\coth(\kappa_i) - 1/\kappa_i], \quad (\text{S4})$$

Our goal is to determine the effective persistence length of a homogeneous reference chain with the same conformational chain properties than the heterogeneous chains, averaged over the disorder.

## B. Ansatz

We use the notation  $\int \mathcal{D}R \dots = \iiint d^2u_1 d^2u_2 \dots d^2u_{N-1} \dots$ . The partition function of a chain with fixed  $\kappa_i$  can then be written as

$$\mathcal{Z} = \int \mathcal{D}R \exp \left[ -\sum_i \kappa_i (1 - \mathbf{u}_i \cdot \mathbf{u}_{i+1}) \right] \quad (\text{S5})$$

and the corresponding free energy is  $F = k_B T \log(\mathcal{Z})$ . The disorder average of an observable  $O$  over all possible  $\kappa_i$  is then generally defined in our system as

$$\langle O \rangle_{\text{dis}} = \left[ \prod_{i=1}^{N-1} \int d\kappa_i P(\kappa_i) \right] \int \mathcal{D}R_1 O \exp \left[ - \sum_i^{N-1} \kappa_i (1 - \mathbf{u}_i \cdot \mathbf{u}_{i+1}) \right] / \mathcal{Z}(\kappa_i). \quad (\text{S6})$$

We need to calculate the disorder averaged free energy,  $\langle F \rangle_{\text{dis}} = k_B T \langle \log(\mathcal{Z}) \rangle_{\text{dis}}$ . To this end, we use the Replica trick which is commonly used in disordered systems, and exploit the relation

$$\langle \log(\mathcal{Z}) \rangle_{\text{dis}} = \lim_{m \rightarrow 0} \frac{\langle \mathcal{Z}^m \rangle_{\text{dis}} - 1}{m}. \quad (\text{S7})$$

This leaves us with the task to calculate the averaged partition function for  $m$  chains with identical realization of the disorder,

$$\langle \mathcal{Z}^m \rangle_{\text{dis}} = \left[ \prod_{i=1}^{N-1} \int d\kappa_i P(\kappa_i) \right] \int \mathcal{D}R_1 \dots \mathcal{D}R_m \exp \left[ - \sum_l^{N-1} \kappa_l \sum_{\alpha=1}^m \left( 1 - \mathbf{u}_l^{(\alpha)} \cdot \mathbf{u}_{l+1}^{(\alpha)} \right) \right] \quad (\text{S8})$$

$$= \int \mathcal{D}R_1 \dots \mathcal{D}R_m \exp \left[ - \kappa_0 \sum_{l\alpha} \left( 1 - \mathbf{u}_l^{(\alpha)} \cdot \mathbf{u}_{l+1}^{(\alpha)} \right) \right] \times \left\{ \prod_{i=1}^{N-1} \int d\xi_i P(\xi_i + \kappa_0) \exp \left[ - \xi_i \sum_{\alpha} \left( 1 - \mathbf{u}_i^{(\alpha)} \cdot \mathbf{u}_{i+1}^{(\alpha)} \right) \right] \right\} \quad (\text{S9})$$

$$= \int \mathcal{D}R_1 \dots \mathcal{D}R_m \exp \left[ - \kappa_0 \sum_{i\alpha} \left( 1 - \mathbf{u}_i^{(\alpha)} \cdot \mathbf{u}_{i+1}^{(\alpha)} \right) \right] \times \exp \left[ \frac{\sigma^2}{2} \sum_{i\alpha\beta} \left( 1 - \mathbf{u}_i^{(\alpha)} \cdot \mathbf{u}_{i+1}^{(\alpha)} \right) \left( 1 - \mathbf{u}_i^{(\beta)} \cdot \mathbf{u}_{i+1}^{(\beta)} \right) \right] \quad (\text{S10})$$

where we use  $\kappa_i = \kappa_0 + \xi_i$  and  $\int_{-\infty}^{\infty} \exp[-(ax^2 + bx)] dx = \sqrt{\pi/a} \exp[b^2/(4a)]$  with  $a = 1/(2\sigma^2)$  and  $b = \sum_{\alpha} (1 - \mathbf{u}_i^{(\alpha)} \cdot \mathbf{u}_{i+1}^{(\alpha)})$ . The corresponding quantity for the homogeneous reference chain is

$$\mathcal{Z}_{\text{ref}} = \int \mathcal{D}R_1 \dots \mathcal{D}R_m \exp \left[ - \kappa_{\text{eff}} \sum_{i\alpha} \left( 1 - \mathbf{u}_i^{(\alpha)} \cdot \mathbf{u}_{i+1}^{(\alpha)} \right) \right]$$

where  $\kappa_{\text{eff}}$  is the angle potential parameter of the reference chain. Subtracting the two from each other, we obtain

$$\begin{aligned} \langle \mathcal{Z}^m - \mathcal{Z}_{\text{ref}}^m \rangle_{\text{dis}} &= \int \mathcal{D}R_1 \dots \mathcal{D}R_m \exp \left[ - \kappa_{\text{eff}} \sum_{i\alpha} \left( 1 - \mathbf{u}_i^{(\alpha)} \cdot \mathbf{u}_{i+1}^{(\alpha)} \right) \right] \\ &\times \left\{ \exp \left[ (\kappa_{\text{eff}} - \kappa_0) \sum_{i\alpha} \left( 1 - \mathbf{u}_i^{(\alpha)} \cdot \mathbf{u}_{i+1}^{(\alpha)} \right) \right] \exp \left[ \frac{\sigma^2}{2} \sum_{i\alpha\beta} \left( 1 - \mathbf{u}_i^{(\alpha)} \cdot \mathbf{u}_{i+1}^{(\alpha)} \right) \left( 1 - \mathbf{u}_i^{(\beta)} \cdot \mathbf{u}_{i+1}^{(\beta)} \right) \right] - 1 \right\}. \end{aligned} \quad (\text{S11})$$

Using the notation

$$\langle A \rangle_{\kappa_{\text{eff}}} = \frac{\int \mathcal{D}R_1 \dots \mathcal{D}R_m \exp \left[ -\kappa_{\text{eff}} \sum_{i\alpha} \left( 1 - \mathbf{u}_i^{(\alpha)} \cdot \mathbf{u}_{i+1}^{(\alpha)} \right) \right] A}{\mathcal{Z}_{\text{ref}}} \quad (\text{S12})$$

we can rewrite this to:

$$\begin{aligned} \langle \mathcal{Z}^m - \mathcal{Z}_{\text{ref}}^m \rangle_{\text{dis}} &= \mathcal{Z}_{\text{ref}}^m \left\langle \exp \left[ (\kappa_{\text{eff}} - \kappa_0) \sum_{i\alpha} \left( 1 - \mathbf{u}_i^{(\alpha)} \cdot \mathbf{u}_{i+1}^{(\alpha)} \right) \right] \right. \\ &\quad \times \exp \left[ \frac{\sigma^2}{2} \sum_{i\alpha\beta} \left( 1 - \mathbf{u}_i^{(\alpha)} \cdot \mathbf{u}_{i+1}^{(\alpha)} \right) \left( 1 - \mathbf{u}_i^{(\beta)} \cdot \mathbf{u}_{i+1}^{(\beta)} \right) \right] - 1 \left. \right\rangle_{\kappa_{\text{eff}}} . \end{aligned}$$

We note that  $\langle O \rangle_{\kappa_{\text{eff}}}$  denotes a pure *thermal* average for fixed given parameter  $\kappa_{\text{eff}}$ , different from  $\langle O \rangle_{\text{dis}}$ , which also includes a disorder average over  $\kappa_i$ .

Now we Taylor expand the averages and get

$$\begin{aligned} \langle \mathcal{Z}^m - \mathcal{Z}_{\text{ref}}^m \rangle_{\text{dis}} &\approx \mathcal{Z}_{\text{ref}}^m \left[ (\kappa_{\text{eff}} - \kappa_0) \sum_{i\alpha} \left\langle \left( 1 - \mathbf{u}_i^{(\alpha)} \cdot \mathbf{u}_{i+1}^{(\alpha)} \right) \right\rangle_{\kappa_{\text{eff}}} \right. \\ &\quad \left. + \frac{\sigma^2}{2} \sum_{i\alpha\beta} \left\langle \left( 1 - \mathbf{u}_i^{(\alpha)} \cdot \mathbf{u}_{i+1}^{(\alpha)} \right) \left( 1 - \mathbf{u}_i^{(\beta)} \cdot \mathbf{u}_{i+1}^{(\beta)} \right) \right\rangle_{\kappa_{\text{eff}}} \right] \\ &= \mathcal{Z}_{\text{ref}}^m N \left[ (\kappa_{\text{eff}} - \kappa_0) m v_1(\kappa_{\text{eff}}) + \frac{\sigma^2}{2} (m^2 v_1(\kappa_{\text{eff}})^2 + m (v_2(\kappa_{\text{eff}}) - v_1(\kappa_{\text{eff}})^2)) \right]. \end{aligned}$$

Here we have defined  $v_n = \left\langle \left( 1 - \mathbf{u}_i^{(\alpha)} \cdot \mathbf{u}_{i+1}^{(\alpha)} \right)^n \right\rangle_{\kappa_{\text{eff}}}$ . Specifically, inserting the angular potential above, we get

$$\begin{aligned} Z(\kappa) &= \int_0^\pi \exp[-\kappa(1 - \cos(\theta))] \sin(\theta) d\theta = \frac{1 - e^{-2\kappa}}{\kappa} \\ P(\theta, \kappa) &= \frac{1}{Z(\kappa)} \exp[-\kappa(1 - \cos(\theta))] \\ v_1(\kappa_{\text{eff}}) &= \int_0^\pi P(\theta, \kappa_{\text{eff}}) [1 - \cos(\theta)] \sin(\theta) d\theta = 1 + \frac{1}{\kappa_{\text{eff}}} - \coth(\kappa_{\text{eff}}) \\ v_2(\kappa_{\text{eff}}) &= \int_0^\pi P(\theta, \kappa_{\text{eff}}) [1 - \cos(\theta)]^2 \sin(\theta) d\theta \\ &= \frac{2}{\kappa_{\text{eff}}^2} + 2 \frac{1 + \kappa_{\text{eff}}}{\kappa_{\text{eff}}} [1 - \coth(\kappa_{\text{eff}})] \\ v_n(\kappa_{\text{eff}}) &= \int_0^\pi P(\theta, \kappa_{\text{eff}}) [1 - \cos(\theta)]^n \sin(\theta) d\theta \\ &= \frac{\exp(2\kappa_{\text{eff}}) \kappa_{\text{eff}}^{-n} [\Gamma(1+n) - \Gamma(1+n, 2\kappa_{\text{eff}})]}{\exp(2\kappa_{\text{eff}}) - 1} \end{aligned}$$

Inserting these results, we can calculate the free energy difference between the disorder averaged heterogeneous chain and the reference chain

$$\Delta F = \lim_{m \rightarrow 0} \frac{\langle \mathcal{Z}^m - \mathcal{Z}_{\text{ref}}^m \rangle_{\text{dis}}}{m} = N \left[ v_1(\kappa_{\text{eff}}) (\kappa_{\text{eff}} - \kappa_0) + \frac{\sigma_\kappa^2}{2} (v_2(\kappa_{\text{eff}}) - v_1(\kappa_{\text{eff}})^2) \right]. \quad (\text{S13})$$

Now we optimize the reference system such that  $\Delta F = 0$ , which gives the following implicit equation for  $\kappa_{\text{eff}}$ :

$$\kappa_{\text{eff}} = \kappa_0 - \frac{\sigma_\kappa^2}{2} h(\kappa_{\text{eff}}) \quad (\text{S14})$$

with

$$h(\kappa) = \frac{v_2(\kappa) - v_1(\kappa)^2}{v_1(\kappa)} = \frac{1 - \kappa^2 / \sinh(\kappa)^2}{\kappa [1 + \kappa - \kappa \coth(\kappa)]} \quad (\text{S15})$$

For small and large  $\kappa$  the function  $f(\kappa)$  has the limiting behavior

$$h(\kappa) \approx \begin{cases} \frac{1}{3} + \frac{\kappa}{9} & (\kappa < 1) \\ \frac{1}{\kappa} & (\kappa > 1) \end{cases} \quad (\text{S16})$$

### C. Effective persistence length

Summarizing the previous subsections: We consider a (quenched) ensemble of heterogeneous semiflexible chains with angle potential parameters  $\kappa_i$ , which are Gaussian distributed with mean  $\kappa_0$  and variance  $\sigma_\kappa$ . According to the above theoretical calculation, the configurational properties should have the same distribution than a reference chain with the renormalized angle potential parameter

$$\kappa_{\text{eff}} / \kappa_0 = 1 - \frac{\sigma_\kappa^2}{2\kappa_0} h(\kappa_{\text{eff}}) \stackrel{\kappa \gg 4}{\approx} 1 - \frac{1}{2} \left( \frac{\sigma_\kappa}{\kappa_0} \right)^2 \quad (\text{S17})$$

Now, instead of looking at the heterogeneously distributed angular potential parameter, we consider the persistence length  $\ell_{p,i} = \ell_p(\kappa_i)$  with

$$\ell_p(\kappa) = \frac{-b}{\log(\langle \cos(\theta) \rangle)} = \frac{-b}{\log[\coth(\kappa) - 1/\kappa]} \stackrel{\kappa \gg 4}{\approx} b \left( \kappa - \frac{1}{2} \right). \quad (\text{S18})$$

The set of local persistence lengths of the Gaussian distributed  $\kappa$  values follow the distribution  $P(\ell_p)$  with mean  $\langle \ell_p \rangle_{\text{dis}}$ . Taylor expanding  $\ell_p(\kappa)$  and using the Gaussian integral identities

$$\int_{-\infty}^{\infty} dx \frac{1}{\sqrt{2\pi}\sigma} \exp\left[\frac{(x-\mu)^2}{2\sigma^2}\right] (x-\mu)^n = \begin{cases} 0 & , n \text{ is odd} \\ 1 & , n = 0 \\ \sigma^2 & , n = 2 \\ 3\sigma^4 & , n = 4 \end{cases} \quad (\text{S19})$$

we can approximate  $\langle \ell_p \rangle_{\text{dis}}$  by:

$$\begin{aligned} \langle \ell_p \rangle_{\text{dis}} &= \int d\kappa P(\kappa) \ell_p(\kappa) \\ &\approx \int d\kappa P(\kappa) \left[ \ell_p(\kappa_0) + \ell'_p(\kappa_0)(\kappa - \kappa_0) + \frac{1}{2} \ell''_p(\kappa_0)(\kappa - \kappa_0)^2 \right] \\ &\approx \ell(\kappa_0) + \frac{1}{2} \ell''_p(\kappa_0) \sigma_\kappa^2. \end{aligned} \quad (\text{S20})$$

Furthermore, since

$$\begin{aligned} \langle \ell_p^2 \rangle_{\text{dis}} &= \int d\kappa P(\kappa) \ell_p(\kappa)^2 \\ &\approx \int d\kappa P(\kappa) \left[ \ell_p(\kappa_0) + \ell'_p(\kappa_0)(\kappa - \kappa_0) + \frac{1}{2} \ell''_p(\kappa_0)(\kappa - \kappa_0)^2 \right]^2 \\ &\approx \ell_p(\kappa_0)^2 + \sigma_\kappa^2 \left[ \ell'_p(\kappa_0)^2 + \ell_p(\kappa_0) \ell''_p(\kappa_0) \right], \end{aligned}$$

the distribution has the variance (up to order  $\sigma_\kappa^2$ )

$$\sigma_p^2 = \langle \ell_p^2 \rangle_{\text{dis}} - \langle \ell_p \rangle_{\text{dis}}^2 = \ell'_p(\kappa_0)^2 \sigma_\kappa^2. \quad (\text{S21})$$

We combine this with Equation (S20) and obtain the following implicit equation for  $\langle \ell_p \rangle_{\text{dis}}$  as a function of  $\kappa_0$  and  $\sigma_p^2$ :

$$\langle \ell_p \rangle_{\text{dis}} = \ell_p(\kappa_0) + \frac{1}{2} \frac{\ell''_p(\kappa_0)}{\ell'_p(\kappa_0)^2} \sigma_p^2. \quad (\text{S22})$$

The persistence length of the reference chain is given by  $\ell_{p,\text{eff}} = \ell_p(\kappa_{\text{eff}})$ . Compared to  $\langle \ell_p \rangle_{\text{dis}}$ , it is shifted by

$$\begin{aligned} \ell_{p,\text{eff}} - \langle \ell_p \rangle_{\text{dis}} &= \left[ \ell_p(\kappa_0) + \ell'_p(\kappa_0)(\kappa_{\text{eff}} - \kappa_0) \right] - \left[ \ell_p(\kappa_0) + \frac{1}{2} \ell''_p(\kappa_0) \sigma_\kappa^2 \right] \\ &\stackrel{\text{eq. S14}}{=} -\frac{\sigma_\kappa^2}{2} \left[ \ell'_p(\kappa_0) h(\kappa_{\text{eff}}) + \ell''_p(\kappa_0) \right] \\ &\stackrel{h(\kappa_{\text{eff}}) \approx h(\kappa_0)}{=} -\frac{\sigma_\kappa^2}{2} \left[ \ell'_p(\kappa_0) h(\kappa_0) + \ell''_p(\kappa_0) \right] \\ &\stackrel{\text{eq. S21}}{=} -\frac{\sigma_p^2}{2} \left[ h(\kappa_0) / \ell'_p(\kappa_0) + \ell''_p(\kappa_0) / \ell'_p(\kappa_0)^2 \right] \end{aligned}$$

Using Equation (S22), we can also express  $\ell_{\text{p,eff}}$  as

$$\ell_{\text{p,eff}} = \ell_{\text{p}}(\kappa_0) - \frac{\sigma_{\text{p}}^2}{2} \frac{h(\kappa_0)}{\ell'_{\text{p}}(\kappa_0)} \quad (\text{S23})$$

If  $\kappa_0 > 4$ , we can use the approximation  $\ell_{\text{p}}(\kappa) \approx b(\kappa - 1/2)$  giving  $\ell''_{\text{p}}(\kappa_0) \approx 0$ , and  $h(\kappa) \approx 1/\kappa$ . Equation (S23) then simplifies like

$$\langle \ell_{\text{p}} \rangle_{\text{dis}} \approx \ell_{\text{p}}(\kappa_0) \quad (\text{S24})$$

$$\ell_{\text{p,eff}} \approx \langle \ell_{\text{p}} \rangle_{\text{dis}} - \frac{\sigma_{\text{p}}^2}{2} \frac{1}{\kappa_0 \ell'_{\text{p}}(\kappa_0)} \quad (\text{S25})$$

$$\approx \langle \ell_{\text{p}} \rangle_{\text{dis}} - \frac{\sigma_{\text{p}}^2}{2} \frac{1}{\left(\frac{\ell_{\text{p}}(\kappa)}{b} + \frac{1}{2}\right) b} \quad (\text{S26})$$

$$\approx \langle \ell_{\text{p}} \rangle_{\text{dis}} - \frac{\sigma_{\text{p}}^2}{2 \langle \ell_{\text{p}} \rangle_{\text{dis}} + b} \quad (\text{S27})$$

#### D. Generalization to higher orders

Here, we derive a higher order expression starting from Eq. (S13). For convenience, we define the shortcut notation  $\gamma = 1 - \cos(\theta)$  and denote  $\gamma_{\alpha}^{(i)} = 1 - \cos(\theta_{i,i+1}^{(\alpha)}) = 1 - \mathbf{u}_i^{(\alpha)} \cdot \mathbf{u}_{i+1}^{(\alpha)}$  etc. We first consider for some given fixed  $i$  the simpler average

$$\left\langle \exp \left( \varepsilon \sum_{\alpha} \gamma_{\alpha} \right) \right\rangle_{\kappa_{\text{eff}}} = \prod_{\alpha} \langle \exp(\varepsilon \gamma_{\alpha}) \rangle_{\kappa_{\text{eff}}} = \langle \exp(\varepsilon \gamma) \rangle_{\kappa_{\text{eff}}}^m, \quad (\text{S28})$$

where we have dropped the superscript  $(i)$  for simplicity. The relation is valid because the  $\gamma_{\alpha}$  are statistically independent for different  $\alpha$ . We can express  $\langle \exp(\varepsilon \gamma) \rangle_{\kappa_{\text{eff}}}$  in terms of a cumulant expansion

$$\langle \exp(\varepsilon \gamma) \rangle_{\kappa_{\text{eff}}} = \exp \left( \sum_{n=0}^{\infty} \frac{\varepsilon^n}{n!} C_{\gamma}^{(n)} \right) \quad (\text{S29})$$

with cumulants  $C_\gamma^{(n)}$  evaluated with respect to  $\langle \cdot \rangle_{\kappa_{\text{eff}}}$  according to<sup>2</sup>

$$C_\gamma^{(n)} = (-1)^{n+1} \begin{vmatrix} v_1 & 1 & 0 & 0 & 0 & 0 & \dots & 0 \\ v_2 & v_1 & 1 & 0 & 0 & 0 & \dots & 0 \\ v_3 & v_2 & \binom{2}{1} v_1 & 1 & 0 & 0 & \dots & 0 \\ v_4 & v_3 & \binom{3}{1} v_2 & \binom{3}{2} v_1 & 1 & 0 & \dots & 0 \\ v_5 & v_4 & \binom{4}{1} v_3 & \binom{4}{2} v_2 & \binom{4}{3} v_1 & 1 & \dots & 0 \\ \dots & \dots \\ v_{n-1} & v_{n-2} & \dots & \dots & \dots & \dots & \dots & 1 \\ v_n & v_{n-1} & \dots & \dots & \dots & \dots & \dots & \binom{n-1}{n-2} v_1 \end{vmatrix} \quad (\text{S30})$$

with  $v_n = \langle \gamma^n \rangle_{\kappa_{\text{eff}}}$ , i.e.,

$$C_\gamma^{(1)} = \langle \gamma \rangle_{\kappa_{\text{eff}}} = v_1 \quad (\text{S31})$$

$$C_\gamma^{(2)} = \langle (\gamma - \langle \gamma \rangle_{\kappa_{\text{eff}}})^2 \rangle_{\kappa_{\text{eff}}} = v_2 - v_1^2 \quad (\text{S32})$$

$$C_\gamma^{(3)} = \langle (\gamma - \langle \gamma \rangle_{\kappa_{\text{eff}}})^3 \rangle_{\kappa_{\text{eff}}} = v_3 - 3v_2v_1 + 2v_1^3 \quad (\text{S33})$$

etc. On the other hand, we can also expand directly

$$\left\langle \exp \left( \varepsilon \sum_{\alpha} \gamma_{\alpha} \right) \right\rangle_{\kappa_{\text{eff}}} = \sum_{n=0}^{\infty} \frac{\varepsilon^n}{n!} \left\langle \left( \sum_{\alpha} \gamma_{\alpha} \right)^n \right\rangle_{\kappa_{\text{eff}}} = 1 + \sum_{n=1}^{\infty} \frac{\varepsilon^n}{n!} \sum_{\alpha_1 \dots \alpha_n} \langle \gamma_{\alpha_1} \dots \gamma_{\alpha_n} \rangle_{\kappa_{\text{eff}}} \quad (\text{S34})$$

Comparing both expansions, we see that

$$\begin{aligned} \left\langle \exp \left( \varepsilon \sum_{\alpha} \gamma_{\alpha} \right) \right\rangle_{\kappa_{\text{eff}}} &= 1 + \sum_{n=1}^{\infty} \frac{\varepsilon^n}{n!} \sum_{\alpha_1 \dots \alpha_n} \langle \gamma_{\alpha_1} \dots \gamma_{\alpha_n} \rangle_{\kappa_{\text{eff}}} \\ &= \langle \exp(\varepsilon \gamma) \rangle_{\kappa_{\text{eff}}}^m = \exp \left( m \sum_{n=0}^{\infty} \frac{\varepsilon^n}{n!} C_\gamma^{(n)} \right) \stackrel{\text{Taylor}}{=} 1 + m \sum_{n=0}^{\infty} \frac{\varepsilon^n}{n!} C_\gamma^{(n)} + \mathcal{O}(m^2) \end{aligned} \quad (\text{S35})$$

and hence we obtain, by comparing coefficients of  $\varepsilon^n$ :

$$\sum_{\alpha_1 \dots \alpha_n} \langle \gamma_{\alpha_1} \dots \gamma_{\alpha_n} \rangle_{\kappa_{\text{eff}}} = m C_\gamma^{(n)} + \mathcal{O}(m^2) \quad (\text{S36})$$

which establishes the relation between our problem and the cumulant expansion. Now we can return to the original problem of Eq. (S13), which we rewrite as

$$\begin{aligned}
& \left\langle \exp \left[ \sum_i \left( (\kappa_{\text{eff}} - \kappa_0) \sum_{\alpha} \gamma_{\alpha}^{(i)} + \frac{\sigma_{\kappa}^2}{2} \sum_{\alpha\beta} \gamma_{\alpha}^{(i)} \gamma_{\beta}^{(i)} \right) \right] - 1 \right\rangle_{\kappa_{\text{eff}}} \\
&= \prod_{i=1}^N \left\langle \exp \left[ (\kappa_{\text{eff}} - \kappa_0) \sum_{\alpha} \gamma_{\alpha}^{(i)} + \frac{\sigma_{\kappa}^2}{2} \sum_{\alpha\beta} \gamma_{\alpha}^{(i)} \gamma_{\beta}^{(i)} \right] \right\rangle_{\kappa_{\text{eff}}} - 1 \\
&= \left\langle \exp \left[ (\kappa_{\text{eff}} - \kappa_0) \sum_{\alpha} \gamma_{\alpha} + \frac{\sigma_{\kappa}^2}{2} \sum_{\alpha\beta} \gamma_{\alpha} \gamma_{\beta} \right] \right\rangle_{\kappa_{\text{eff}}}^N - 1,
\end{aligned} \tag{S37}$$

where we have used that the  $\gamma_{\alpha}^{(i)}$  for different  $i$  are statistically independent and have the same distribution function.

We first calculate

$$\begin{aligned}
& \left\langle \exp \left[ (\kappa_{\text{eff}} - \kappa_0) \sum_{\alpha} \gamma_{\alpha} + \frac{\sigma_{\kappa}^2}{2} \sum_{\alpha\beta} \gamma_{\alpha} \gamma_{\beta} \right] \right\rangle_{\kappa_{\text{eff}}} \\
&= \left\langle \exp \left[ (\kappa_{\text{eff}} - \kappa_0) \sum_{\alpha} \gamma_{\alpha} \right] \exp \left[ \frac{\sigma_{\kappa}^2}{2} \sum_{\alpha\beta} \gamma_{\alpha} \gamma_{\beta} \right] \right\rangle_{\kappa_{\text{eff}}} \\
&= \left\langle \sum_{n=0}^{\infty} \frac{(\kappa_{\text{eff}} - \kappa_0)^n}{n!} \sum_{k=0}^{\infty} \frac{(\sigma_{\kappa}^2/2)^k}{k!} \left( \sum_{\alpha} \gamma_{\alpha} \right)^n \left( \sum_{\alpha\beta} \gamma_{\alpha} \gamma_{\beta} \right)^k \right\rangle_{\kappa_{\text{eff}}} \\
&= \sum_{n=0}^{\infty} \sum_{k=0}^{\infty} \frac{(\kappa_{\text{eff}} - \kappa_0)^n}{n!} \frac{(\sigma_{\kappa}^2/2)^k}{k!} \left\langle \left( \sum_{\alpha} \gamma_{\alpha} \right)^n \left( \sum_{\alpha\beta} \gamma_{\alpha} \gamma_{\beta} \right)^k \right\rangle_{\kappa_{\text{eff}}} \\
&= 1 + \sum_{\substack{n,k=0 \\ n+k \geq 1}}^{\infty} \frac{(\kappa_{\text{eff}} - \kappa_0)^n}{n!} \frac{(\sigma_{\kappa}^2/2)^k}{k!} \sum_{\alpha_1 \dots \alpha_n \alpha'_1 \dots \alpha'_k \beta_1 \dots \beta_k} \langle \gamma_{\alpha_1} \dots \gamma_{\beta_k} \rangle_{\kappa_{\text{eff}}}
\end{aligned} \tag{S38}$$

Now, we rewrite the summation in orders of  $\gamma$ 's by converting  $\alpha_1 \dots \alpha_n \alpha'_1 \dots \alpha'_k \beta_1 \dots \beta_k$  to  $\alpha_1 \dots \alpha_l$  leading to a summation shift according to  $l = n + 2k$ .

$$\begin{aligned}
& \left\langle \exp \left[ (\kappa_{\text{eff}} - \kappa_0) \sum_{\alpha} \gamma_{\alpha} + \frac{\sigma_{\kappa}^2}{2} \sum_{\alpha\beta} \gamma_{\alpha} \gamma_{\beta} \right] \right\rangle_{\kappa_{\text{eff}}} \\
&= 1 + \sum_{l=1}^{\infty} \sum_{\alpha_1 \dots \alpha_l} \langle \gamma_{\alpha_1} \dots \gamma_{\alpha_l} \rangle_{\kappa_{\text{eff}}} \sum_{k=0}^{\text{floor}(l/2)} \frac{(\kappa_{\text{eff}} - \kappa_0)^{l-2k}}{k!(l-2k)!} \frac{(\sigma_{\kappa}^2/2)^k}{k!(l-2k)!} \\
&= 1 + m \sum_{l=1}^{\infty} A_l C_{\gamma}^{(l)} + \mathcal{O}(m^2),
\end{aligned} \tag{S39}$$

where we have used Eq. (S36) and defined

$$A_l := \sum_{k=0}^{\text{floor}(l/2)} \frac{(\kappa_{\text{eff}} - \kappa_0)^{l-2k} (\sigma_\kappa^2/2)^k}{k!(l-2k)!}. \quad (\text{S40})$$

For example, we have

$$\begin{aligned} A_1 &= (\kappa_{\text{eff}} - \kappa_0) \\ A_2 &= \frac{1}{2}(\kappa_{\text{eff}} - \kappa_0)^2 + \frac{\sigma_\kappa^2}{2} \\ A_3 &= \frac{1}{6}(\kappa_{\text{eff}} - \kappa_0)^3 + (\kappa_{\text{eff}} - \kappa_0) \frac{\sigma_\kappa^2}{2} \\ A_4 &= \frac{1}{24}(\kappa_{\text{eff}} - \kappa_0)^4 + \frac{1}{2}(\kappa_{\text{eff}} - \kappa_0)^2 \frac{\sigma_\kappa^2}{2} + \frac{1}{2} \left( \frac{\sigma_\kappa^2}{2} \right)^2. \end{aligned}$$

Finally, putting everything together, we obtain

$$\left\langle \exp \left[ \sum_i \left( (\kappa_{\text{eff}} - \kappa_0) \sum_\alpha \gamma_\alpha^{(i)} + \frac{\sigma_\kappa^2}{2} \sum_{\alpha\beta} \gamma_\alpha^{(i)} \gamma_\beta^{(i)} \right) \right] - 1 \right\rangle_{\kappa_{\text{eff}}} \quad (\text{S41})$$

$$= \left( 1 + m \sum_{l=1}^{\infty} A_l C_\gamma^{(l)} + \mathcal{O}(m^2) \right)^N - 1 \stackrel{\mathcal{O}(m)}{=} mN \sum_{l=1}^{\infty} A_l C_\gamma^{(l)} \quad (\text{S42})$$

The “problem” is that all the  $A_l$  depend on powers of  $(\kappa_{\text{eff}} - \kappa_0)$  (up to power  $l$ ) and  $\sigma_\kappa^2/2$  (up to power  $\text{floor}(l/2)$ ). Therefore, determining  $\kappa_{\text{eff}}$  by setting Eq. (S42) to zero requires setting up yet another series. This can be done by an iterative procedure, similar to perturbation theory in quantum mechanics, starting from the equation

$$(\kappa_{\text{eff}} - \kappa_0) = - \sum_{l=2}^{\infty} A_l \frac{C_\gamma^{(l)}}{C_\gamma^{(1)}} \quad (\text{S43})$$

and treating  $\sigma_\kappa^2/2$  as a small parameter. For example, the two first terms in this expansion are

$$(\kappa_{\text{eff}} - \kappa_0) = - \frac{\sigma_\kappa^2}{2} \frac{C_\gamma^{(2)}}{C_\gamma^{(1)}} - \left( \frac{\sigma_\kappa^2}{2} \right)^2 \left[ \frac{1}{2} \left( \frac{C_\gamma^{(2)}}{C_\gamma^{(1)}} \right)^3 - \frac{C_\gamma^{(3)}}{C_\gamma^{(1)}} \frac{C_\gamma^{(2)}}{C_\gamma^{(1)}} \right] + \dots$$

## E. Alternative series approximation

In Eqs. (S38), we have split the exponential functions into two series which are cut off individually when computing the cumulants later on. This gives us a convenient way of

computing  $\sum_{\alpha_1 \dots \alpha_l} \langle \gamma_{\alpha_1} \dots \gamma_{\alpha_l} \rangle_{\kappa_{\text{eff}}} = C_\gamma^{(l)}$  at the cost that we are considering different orders of approximations. Alternatively, one can compute the disorder average as a single exponential series and rewrite its binomial such that one gets the form

$$\begin{aligned} & \left\langle \exp \left[ (\kappa_{\text{eff}} - \kappa_0) \sum_{\alpha} \gamma_{\alpha} + \frac{\sigma_{\kappa}^2}{2} \sum_{\alpha, \beta} \gamma_{\alpha} \gamma_{\beta} \right] \right\rangle_{\kappa_{\text{eff}}} \\ & \approx \sum_{n=0}^{N_{\text{cut}}} \sum_{k=0}^n \binom{n}{k} \left( \frac{(\kappa_{\text{eff}} - \kappa_0)^{n-k}}{n!} \frac{\sigma_{\kappa}^{2k}}{2^k} \left\langle \left( \sum_{\alpha} \gamma_{\alpha} \right)^{n-k} \left( \sum_{\alpha, \beta} \gamma_{\alpha} \gamma_{\beta} \right)^k \right\rangle_{\kappa_{\text{eff}}} \right) \end{aligned} \quad (\text{S44})$$

for which we can identify the different orders of  $(\sigma_{\kappa}^2/2)$  and  $(\kappa_{\text{eff}} - \kappa_0)$  to find the solution of the disorder average according to Eq. (S39). Doing this and considering only orders up to  $m$  in Eq. (S39) we can rewrite (S44) as:

$$\begin{aligned} & \left\langle \exp \left[ (\kappa_{\text{eff}} - \kappa_0) \sum_{\alpha} \gamma_{\alpha} + \frac{\sigma_{\kappa}^2}{2} \sum_{\alpha, \beta} \gamma_{\alpha} \gamma_{\beta} \right] \right\rangle_{\kappa_{\text{eff}}} = 1 + m \sum_{l=1}^{\infty} A_l C_\gamma^{(l)} \\ & = 1 + m \sum_{l=1}^{\infty} \sum_k^{\text{floor}(l/2)} \frac{(\kappa_{\text{eff}} - \kappa_0)^{l-2k} (\sigma_{\kappa}^2/2)^k}{k!(l-2k)!} C_\gamma^{(l)} \\ & = 1 + m \sum_{n=1}^{\infty} \sum_{k=0}^n \frac{(\kappa_{\text{eff}} - \kappa_0)^{n-k} (\sigma_{\kappa}^2/2)^k}{k!(n-k)!} C_\gamma^{(n+k)} \end{aligned}$$

Re-ordered in this way, the series turns out to converge more uniformly than the series presented in Eq. (S39), with convergence properties similar to the exponential function.

## F. Generalization to other distributions

Extending the assumption of  $P(\kappa_i)$  in Eq. (S2) to a weighted sum of normal distributions like

$$P(\kappa_i) = \sum_j^K \frac{\omega_j}{\sqrt{2\pi}\sigma_{\kappa,j}} \exp \left( -\frac{(\kappa_i - \kappa_{0,j})^2}{2\sigma_{\kappa,j}^2} \right) \quad (\text{S45})$$

allows for more heterogeneous polymers, while still being mathematically tractable. Enforcing  $\sum_j^K \omega_j = 1$  conserves  $\int d\kappa_i P(\kappa_i) = 1$ . We write the disorder averaged partition function

of Eq. (S8) as :

$$\begin{aligned}
\langle \mathcal{Z}^m \rangle_{\text{dis}} &= \int \mathcal{D}R_1 \dots \mathcal{D}R_m \prod_{i=1}^{N-1} \int d\kappa_i \left[ \sum_j^K \frac{\omega_j}{\sqrt{2\pi\sigma_{\kappa,j}^2}} \exp\left(-\frac{(\kappa_i - \kappa_{0,j})^2}{2\sigma_{\kappa,j}^2}\right) \right] \exp\left(-\kappa_i \sum_{\alpha} \gamma_{\alpha}^{(i)}\right) \\
&= \int \mathcal{D}R_1 \dots \mathcal{D}R_m \prod_{i=1}^{N-1} \int d\kappa_i \sum_j^K \frac{\omega_j}{\sqrt{2\pi\sigma_{\kappa,j}^2}} \exp\left[-\left(\frac{1}{2\sigma_{\kappa,j}^2} \kappa_i^2 + \left(\sum_{\alpha} \gamma_{\alpha}^{(i)} - \frac{\kappa_{0,j}}{\sigma_{\kappa,j}^2}\right) \kappa_i + \frac{\kappa_{0,j}^2}{2\sigma_{\kappa,j}^2}\right)\right] \\
&= \int \mathcal{D}R_1 \dots \mathcal{D}R_m \prod_{i=1}^{N-1} \sum_j^K \omega_j \exp\left[\frac{\sigma_{\kappa,j}^2}{2} \left(\sum_{\alpha} \gamma_{\alpha}^{(i)} - \frac{\kappa_{0,j}}{\sigma_{\kappa,j}^2}\right)^2 - \frac{\kappa_{0,j}^2}{2\sigma_{\kappa,j}^2}\right] \\
&= \int \mathcal{D}R_1 \dots \mathcal{D}R_m \prod_{i=1}^{N-1} \sum_j^K \omega_j \exp\left(-\kappa_{0,j} \sum_{\alpha} \gamma_{\alpha}^{(i)} + \frac{\sigma_{\kappa,j}^2}{2} \sum_{\alpha,\beta} \gamma_{\alpha}^{(i)} \gamma_{\beta}^{(i)}\right) \\
&= \int \mathcal{D}R_1 \dots \mathcal{D}R_m \exp\left(-\kappa_{\text{eff}} \sum_{\alpha,i} \gamma_{\alpha}^{(i)}\right) \prod_{i=1}^{N-1} \sum_j^K \omega_j \exp\left[-(\kappa_{0,j} - \kappa_{\text{eff}}) \sum_{\alpha} \gamma_{\alpha}^{(i)} + \frac{\sigma_{\kappa,j}^2}{2} \sum_{\alpha,\beta} \gamma_{\alpha}^{(i)} \gamma_{\beta}^{(i)}\right] \\
&= \left\langle \prod_{i=1}^{N-1} \sum_j^K \omega_j \exp\left[-(\kappa_{0,j} - \kappa_{\text{eff}}) \sum_{\alpha} \gamma_{\alpha}^{(i)} + \frac{\sigma_{\kappa,j}^2}{2} \sum_{\alpha,\beta} \gamma_{\alpha}^{(i)} \gamma_{\beta}^{(i)}\right] \right\rangle_{\kappa_{\text{eff}}}
\end{aligned}$$

using  $\int_{-\infty}^{\infty} \exp[-(ax^2 + bx + c)] dx = \sqrt{\pi/a} \exp[b^2/(4a) - c]$  with  $a = 1/(2\sigma_{\kappa,j}^2)$ ,  $b = \sum_{\alpha} \gamma_{\alpha}^{(i)} - \kappa_{0,j}/(\sigma_{\kappa,j}^2)$  and  $c = \kappa_{0,j}^2/(2\sigma_{\kappa,j}^2)$ . This yields

$$\begin{aligned}
\langle \mathcal{Z}^m - \mathcal{Z}_{\text{ref}}^m \rangle_{\text{dis}} &= \left\langle \prod_{i=1}^{N-1} \sum_j^K \omega_j \exp\left[-(\kappa_{0,j} - \kappa_{\text{eff}}) \sum_{\alpha} \gamma_{\alpha}^{(i)} + \frac{\sigma_{\kappa,j}^2}{2} \sum_{\alpha,\beta} \gamma_{\alpha}^{(i)} \gamma_{\beta}^{(i)}\right] - 1 \right\rangle_{\kappa_{\text{eff}}} \\
&= \left\langle \sum_j^K \omega_j \exp\left[-(\kappa_{0,j} - \kappa_{\text{eff}}) \sum_{\alpha} \gamma_{\alpha} + \frac{\sigma_{\kappa,j}^2}{2} \sum_{\alpha,\beta} \gamma_{\alpha} \gamma_{\beta}\right] \right\rangle_{\kappa_{\text{eff}}}^{N-1} - 1
\end{aligned}$$

since the  $\gamma^{(i)}$  are independent from each other. Following Eq. (S44), we can approximate the average by

$$\begin{aligned}
&\left\langle \sum_j^K \omega_j \exp\left[-(\kappa_{0,j} - \kappa_{\text{eff}}) \sum_{\alpha} \gamma_{\alpha} + \frac{\sigma_{\kappa,j}^2}{2} \sum_{\alpha,\beta} \gamma_{\alpha} \gamma_{\beta}\right] \right\rangle_{\kappa_{\text{eff}}} \\
&\approx \sum_{n=0}^{N_{\text{cut}}} \sum_{k=0}^n \sum_j^K \omega_j \binom{n}{k} \left( \frac{(\kappa_{\text{eff}} - \kappa_{0,j})^{n-k}}{n!} \frac{\sigma_{\kappa,j}^{2k}}{2^k} \left\langle \left( \sum_{\alpha} \gamma_{\alpha} \right)^{n-k} \left( \sum_{\alpha,\beta} \gamma_{\alpha} \gamma_{\beta} \right)^k \right\rangle_{\kappa_{\text{eff}}} \right)
\end{aligned}$$

Using our previous results, we can evaluate this finally to

$$\begin{aligned} & \left\langle \sum_j^K \omega_j \exp \left[ -(\kappa_{0,j} - \kappa_{\text{eff}}) \sum_{\alpha} \gamma_{\alpha} + \frac{\sigma_{\kappa,j}^2}{2} \sum_{\alpha,\beta} \gamma_{\alpha} \gamma_{\beta} \right] \right\rangle_{\kappa_{\text{eff}}} \\ &= mN \sum_{n=1}^{N_{\text{cut}}} \sum_{k=0}^n \frac{C_{\gamma}^{(n+k)}}{(n-k)!k!} \sum_j^K \omega_j \left[ (\kappa_{\text{eff}} - \kappa_{0,j})^{n-k} \left( \frac{\sigma_{\kappa,j}^2}{2} \right)^k \right] + \mathcal{O}(m^2) \end{aligned}$$

From this, we compute the difference of the free energy as before.

$$\Delta F = \lim_{m \rightarrow 0} \frac{\langle \mathcal{Z}^m - \mathcal{Z}_{\text{ref}}^m \rangle_{\text{dis}}}{m} = N \sum_{n=1}^{N_{\text{cut}}} \sum_{k=0}^n \frac{C_{\gamma}^{(n+k)}}{(n-k)!k!} \sum_j^K \omega_j \left[ (\kappa_{\text{eff}} - \kappa_{0,j})^{n-k} \left( \frac{\sigma_{\kappa,j}^2}{2} \right)^k \right] \quad (\text{S46})$$

Taking only terms up to order  $n = 2$  in Eq. (S46) and requiring  $\Delta F = 0$ , we obtain

$$\begin{aligned} 0 \approx & C_{\gamma}^{(1)}(\kappa_{\text{eff}} - \kappa_0) + \frac{C_{\gamma}^{(2)}}{2} \sum_j^K \omega_j (\sigma_{\kappa,j}^2 + (\kappa_{\text{eff}} - \kappa_{0,j})^2) + \frac{C_{\gamma}^{(3)}}{2} \sum_j^K \omega_j (\kappa_{\text{eff}} - \kappa_{0,j}) \sigma_{\kappa,j}^2 \\ & + \frac{C_{\gamma}^{(4)}}{4} \sum_j^K \omega_j \sigma_{\kappa,j}^4 = (\kappa_{\text{eff}} - \kappa_0) \left( C_{\gamma}^{(1)} + \frac{C_{\gamma}^{(3)}}{2} \sum_j^K \sigma_{\kappa,j}^2 \right) + (\kappa_{\text{eff}} - \kappa_0)^2 \frac{C_{\gamma}^{(2)}}{2} \\ & + \frac{C_{\gamma}^{(2)}}{2} \sum_j^K \omega_j (\sigma_{\kappa,j}^2 + (\kappa_0 - \kappa_{0,j})^2) + \frac{C_{\gamma}^{(3)}}{2} \sum_j^K \omega_j (\kappa_0 - \kappa_{0,j}) \sigma_{\kappa,j}^2 - \frac{C_{\gamma}^{(4)}}{4} \sum_j^K \omega_j \sigma_{\kappa,j}^4, \quad (\text{S47}) \end{aligned}$$

where we have defined  $\kappa_0 := \sum_j^K \omega_j \kappa_{0,j}$  and used  $\sum_j^K \omega_j (\kappa_0 - \kappa_{0,j}) = 0$ . Our goal is to calculate the difference between the effective bending parameter,  $\kappa_{\text{eff}}$ , and the average bending parameter,  $\kappa_0 := \sum_j^K \omega_j \kappa_{0,j}$  as a function of  $\sigma_{\kappa,j}$  and  $(\kappa_0 - \kappa_{0,j})$ , which are assumed to be small and of similar order,  $\sigma_{\kappa,j} \sim \varepsilon$  and  $(\kappa_0 - \kappa_{0,j}) \sim \varepsilon$  with  $\varepsilon$  being a small parameter. Therefore, we only keep the leading term in  $(\kappa_{\text{eff}} - \kappa_0)$ , resulting in

$$\begin{aligned} (\kappa_{\text{eff}} - \kappa_0) &= -\frac{1}{C_{\gamma}^{(1)} + \frac{C_{\gamma}^{(3)}}{2} \sum_j^K \sigma_{\kappa,j}^2} \left( \frac{C_{\gamma}^{(2)}}{2} \sum_j^K \omega_j (\sigma_{\kappa,j}^2 + (\kappa_0 - \kappa_{0,j})^2) + \frac{C_{\gamma}^{(3)}}{2} \sum_j^K \omega_j (\kappa_0 - \kappa_{0,j}) \sigma_{\kappa,j}^2 \right) \\ &\approx -\frac{1}{C_{\gamma}^{(1)}} \left( \frac{C_{\gamma}^{(2)}}{2} \sum_j^K \omega_j (\sigma_{\kappa,j}^2 + (\kappa_0 - \kappa_{0,j})^2) + \frac{C_{\gamma}^{(3)}}{2} \sum_j^K \omega_j (\kappa_0 - \kappa_{0,j}) \sigma_{\kappa,j}^2 \right) + \mathcal{O}(\sigma_{\kappa,j}^4) \\ &\approx -\frac{h(\kappa_{\text{eff}})}{2} \sum_j^K \omega_j (\sigma_{\kappa,j}^2 + (\kappa_0 - \kappa_{0,j})^2) + \mathcal{O}(\varepsilon^3). \quad (\text{S48}) \end{aligned}$$

Note that  $(\kappa_{\text{eff}} - \kappa_0)$  is of order  $\varepsilon^2$  according to this expansion, therefore the neglected term  $(\kappa_{\text{eff}} - \kappa_0)^2 C_{\gamma}^{(2)}/2$  in Eq. (S47) is of order  $\varepsilon^4$  and the expansion is consistent. Finally, we note that  $h(\kappa_{\text{eff}})$  can be expanded as  $h(\kappa_{\text{eff}}) \approx h(\kappa_0) + h'(\kappa_0)(\kappa_{\text{eff}} - \kappa_0) = h(\kappa_0) + \mathcal{O}(\varepsilon^2)$  and

obtain

$$\kappa_{\text{eff}} = \kappa_0 - \frac{h(\kappa_0)}{2} \sum_j^K \omega_j [\sigma_{\kappa,j}^2 + (\kappa_0 - \kappa_{0,j})^2] + \mathcal{O}(\varepsilon^3). \quad (\text{S49})$$

Accounting for higher orders of  $n$  in Eq. (S46) does not change this result.

## II. SEQUENCES

1|DSHAKRHHGY KRKFHEKHHS HRGY

(a) **Hst5:**

1|DSHAKRHHGY KRKFHEKHHS HRGYDSHAKR HHGYKRKFHE KHSHRGY

(b) **Hst52:**

1|GPGSDLWKLL PENNVLSPLP SQAMDDLMLS PDDIEQWFTE DPGPDEAPRM PEAALEHHHH  
61|HH

(c) **p532070:**

1|GTQNRPLL RN SLDDL VGPPS NLEGQSDERA LLDQLHTLLS NTDATGLEEI DRALGIPELV  
61|NQGQALEPKQ D

(d) **ACTR:**

1|MSRAALPSLE NLEDDDEFED FATENWPMKD TELDTGDDTL WENNWDDEDI GDDDFSVQLQ  
61|AELKKKGVA A C

(e) **DSS1:**

1|SASSSPSPST PTKSGKMRSR SSSPVRPKAY TPSPRSPNYH RFALDSPPQS PRRSSNSSIT  
61|KKGSRSSGS SPTRHTTRVC V

(f) **Ash1:**

1|FAGSGSNIYS PGNAYSPSS NYSPNSPSYS PTSPSYSPSS PSYSPTSPCY SPTSPSYSP  
61|SPNYTPVTPS YSPTSPNYSA SPQ

(g) **CTD2:**

1|GSMTPTPPR SRGTRYLAQP SGN TSSSALM QGQKTPQKPS QNLVPVTPST TKSFKNAPLL  
61|APPNSNMGMT SPFNGLTSPQ RSPFPKSSVK RT

(h) **Sic1:**

1|MGSNKSKPKD ASQRRRSLEP AENVHGAGGG AFPASQTPSK PASADGHRGP SAAFAPAAAE  
61|PKLFGGFNSS DTVTSPQRAG PLAGGSAWSH PQFEK

(i) **SH4UD:**

1|MGSNGADNAH NNAFGGKNP GIGNTSGAGS NGSASSNRGN SNGWSWSNKP HKNDGFHSDG  
61|SYHITFHGDN NSKPKPGGNS GNRGNNGDGA SSHHHHHH

(j) **ColNT:**

1|GSHMKGACIV ANSPDDVKS KEDVPQTDPR LTGGDRDNAR ASRTGNDPAG ASTQSAEVAC  
61|SNPILSTPDA QEKQAGTSNS KERPHEQLSA GSVEQTPKKP GLRRRQT

(a) **p27Cv15:**

1|GSHMKGACKV PAQESQDVSG SRPAAPLIGA PANSEDTHLV DPKTDPDSQ TGLAEQCAGI  
61|RKRPTDDSS TQNKRRNRTE ENVSDGSPNA GSVEQTPKKP GLRRRQT

(b) **p27Cv31:**

1|GSHMKGACRK PANAEADSSS CQNVPRGKSK QAPETPTGSP LGDATLNQVK PRRPSSASTN  
61|IGQLEDADED DAEDHVGS AV TSQTIPNDRA GSVEQTPKKP GLRRRQT

(c) **p27Cv44:**

1|GSHMKGACGS SVLGTGNPRN QAHVSDTSLE EDDDEQDDST PDEVQACTI VASALDINAA  
61|TPRSPKASPK RKRKRQSTAP AQGNEPPGNA GSVEQTPKKP GLRRRQT

(d) **p27Cv56:**

1|GSHMKGACAL PSGVPAEDD DDDEEEEDDQ DPAQPQAVQG AAPSSGTNNS QPILPSIAVN  
61|STTGPNSTAG KKKRKRRTTR HSNCATLSSA GSVEQTPKKP GLRRRQT

(e) **p27Cv78:**

1|GSHMKGACKS SSPPSNDQGR PGDPKQVIDK TEVERTQDTS NIQETQSANN SGDPKPSRCD  
61|LAVSGVAAAA LPAPGHANST ARDLTRDEEA GSVEQTPKKP GLRRRQT

(f) **p27Cv14:**

1|MVRTKADSV GTYRKVVAAR APRKVLGSST SATNSTSVSS RKAENKYAGG NPVCVRPTPK  
61|WQKGIGEFFR LSPKDSEKEN QIPEEAGSSG LGKAKRKACP LQPDHTNDEK E

(g) **p15PAF:**

1|GPSDAAVDTS SEITTKDLKE KKEVVEEAEN GRDAPANGNA NEENGEQEAD NEVDEEEEEEG  
61|GEEEEEEEEEG DGEEEDGDED EEAESATGKR AAEDDEDDDV DTKKQKTDED D

(h) **PTMA:**

1|GPPLTTTLPA CCGPIARCLT SPQAYENQEQ LKDDSDSLIL NDGDISLTYG DSTVNTEPAT  
61|SSAPRRFMGN SSEDALDREL AFGDHELVIR GTRLVLPMD SEPLNLLDN TRHGPA

(i) **NHE6cmdd:**

1|MYRKDKRRQE PLRQPSPQRG AWAPELGAAP EEELAALQLG PTHHECEAGP PHDTLRLTAL  
61|PDYTLTLRRS PDDIPLMTPN TITMIPNSLV GLQTLHPYNT FAAGFNSTGL PSHSTTRV

(j) **hNL3cyt:**

1|KETAAAKFER QHMDSSSTAA SSSNYCNQMM KSRNLTKDRC KPVNTFVHES LADVQAVCSQ  
61|KNVACKNGQT NCYQSYSTMS ITDCRETGSS KYPNCAYKTT QANKHIIVAC EGNPYVPVHF  
121|DASV

(k) **RNaseA:**

```

1 | GSMASASSSQ RGRSGSGNFG GGRGGGFGGN DNFGRGGNFS GRGGFGGSRG GGGYGGSGDG
61 | YNGFGNDGSN FGGGGYNNQ SSNFGPMKGG NFGGRSSGPY GGGGQYFAKP RNQGGYGGSS
121 | SSSSYGSGRR F

```

(a) **A1S150:**

```

1 | GSMASASSSQ RGRSGSGNFG GGRGGGFGGN GNFGRGGNFS GRGGFGGSRG GGGYGGSGGG
61 | YNGFGNSGSN FGGGGSYNGF GNYNNQSSNF GPMKGGNFGG RSSGPYGGGG QYFAKPRNQG
121 | GYGGSSSSSS YGSGRRF

```

(b) **M4D:**

```

1 | GSMASASSSQ RGRSGSGNFG GGRGGGYGGN DNGGRGGNYS GRGGFGGSRG GGGYGGSGDG
61 | YNGGGNDGSN YGGGGSYNDS GNYNNQSSNF GPMKGGNYGG RSSGGSGGGG QYGAkPRNQG
121 | GYGGSSSSSS YGSGRRF

```

(c) **M8FP4Y:**

```

1 | GSMASASSSQ RGRSGSGNFG GGRGGGYGGN DNGGRGGNYS GRGGFGGSRG GGGYGGSGDG
61 | YNGGGNDGSN YGGGGSYNDS GNGNNQSSNF GPMKGGNYGG RSSGGSGGGG QYGAkPRNQG
121 | GYGGSSSSSS YGSGRRS

```

(d) **M9FP3Y:**

```

1 | GSMASASSSQ GGSSGSGNFG GGGGGGFGGN DNFGGGGNFS GSGGFGGSGG GGGYGGSGDG
61 | YNGFGNDGSN FGGGGSYNDF GNYNNQSSNF GPMKGGNFGG SSSGPYGGGG QYFAKPGNQG
121 | GYGGSSSSSS YSGGGF

```

(e) **M10R:**

```

1 | GSMASASSSQ GGRSGSGNFG GGRGGGFGGN DNFGGGGNFS GSGGFGGSRG GGGYGGSGDG
61 | YNGFGNDGSN FGGGGSYNDF GNYNNQSSNF GPMKGGNFGG SSSGPYGGGG QYFAKPGNQG
121 | GYGGSSSSSS YSGGRRF

```

(f) **M6R:**

```

1 | GSMASASSSQ RGRSGSGNFG GGRGGGFGGN DNFGRGGNFS GRGGFGGSRG GGGYGGSGDG
61 | YNGFRNDGSN FGGGGRYNDF GNYNNQSSNF GPMKGGNFGG RSSGPYGGGG QYFAKPRNQG
121 | YGGSSSSSS YGSGRRF

```

(g) **P2R:**

```

1 | GSMASASSSQ RGRSGRGNFG GGRGGGFGGN DNFGRGGNFS GRGGFGGSRG GGRYGGSGDR
61 | YNGFGNDGRN FGGGGSYNDF GNYNNQSSNF GPMKGGNFRG RSSGPYGRGG QYFAKPRNQG
121 | GYGGSSSSRS YGSGRRF

```

(h) **P7R:**

```

1 | GSMASASSSQ RDRSGSGNFG GGRDGGFGGN DNFGRGDNFS GRGDFGGSRD GGGYGGSGDG
61 | YNGFGNDGSN FGGGGSYNDF GNYNNQSSNF GPMKGGNFGG RSSDPYGGGG QYFAKPRNQD
121 | GYGGSSSSSS YDSGRRF

```

(i) **P8D:**

1 | GSMASADSSQ RDRDDSGNFG DGRGGGFGGN DNFGRGGNFS DRGGFGGSRG DGGYGGDGDG  
61 | YNGFGNDGSN FGGGGSYNDF GNYNNQSSNF DPMKGGNFGD RSSGPYDGGG QYFAKPRNQG  
121 | GYGGSSSSSS YGSDRRF

(a) **P12D:**

1 | GSMASASSSQ RGRSGSGNFG GGRGGGYGGN DNYGRGGNYS GRGGFGGSRG GGGYGGSGDG  
61 | YNGGGNDGSN YGGGGSYNDS GNYNNQSSNF GPMKGGNYGG RSSGGSGGGG QYFAKPRNQG  
121 | GYGGSSSSSS YGSGRRY

(b) **M9FP6Y:**

1 | GSMASASSSQ KGKSGSGNFG GGRGGGFGGN DNFGKGGNFS GRGGFGGSKG GGGYGGSGDG  
61 | YNGFGNDGSN FGGGGSYNDF GNYNNQSSNF GPMKGGNFGG KSSGGSGGGG QYFAKPRNQG  
121 | GYGGSSSSSS YGSGRKF

(c) **M6RP6K:**

1 | GSMASASSSQ RDRSGSGNFG GGRGGGFGGN DNFGRGGNFS GRGDFGGSRG GGGYGGSGDG  
61 | YNGFGNDGSN FGGGGSYNDF GNYNNQSSNF GPMKGGNFGG RSSDPYGGGG QYFAKPRNQG  
121 | GYGGSSSSSS YDSGRRF

(d) **P4D:**

1 | GSMASASSSQ KGKSGSGNFG GGKGGGFGGN DNFGKGGNFS GKGGFGGSKG GGGYGGSGDG  
61 | YNGFGNDGSN FGGGGSYNDF GNYNNQSSNF GPMKGGNFGG KSSGGSGGGG QYFAKPNQG  
121 | GYGGSSSSSS YSGKKF

(e) **M10RP10K:**

1 | GSMASASSSQ RGKSGSGNFG GGRGGGFGGN DNFGRGGNFS GRGGFGGSKG GGGYGGSGDG  
61 | YNGFGNDGSN FGGGGSYNDF GNYNNQSSNF GPMKGGNFGG RSSGGSGGGG QYFAKPRNQG  
121 | GYGGSSSSSS YGSGRKF

(f) **M3RP3K:**

1 | GSMASASSSQ RGRSGSGNFG GGRGGGFGGN DNFGRGGNFS GRGGFGGSRG GGGFGGSGDG  
61 | FNGFGNDGSN FGGGGSFNDF GNFNNQSSNF GPMKGGNFGG RSSGGSGGGG QFFAKPRNQG  
121 | FGSGSSSSSS FGSGRRF

(g) **P7FM7Y:**

1 | GSMASADSSQ RDRDDKGNFG DGRGGGFGGN DNFGRGGNFS DRGGFGGSRG DGKYGGDGDG  
61 | YNGFGNDGKN FGGGGSYNDF GNYNNQSSNF DPMKGGNFKD RSSGPYDKGG QYFAKPRNQG  
121 | GYGGSSSSKS YGSDRRF

(h) **P7KP12D:**

1 | GSMASASSSQ RGRSGSGNFG GGRGGGFGGN DNFGRGGNFS GRGGFGGSRG GGGYGGSGDG  
61 | YNGFGNDGSN FGGGGSYNDF GNYNNQSSNF GPMKGGNFGG RSSGGSGGGG QYFAKPRNQG  
121 | GYGGSSSSSS YGSGRRF

(i) **A1:**

1 | GSMASAKSSQ RDRDDGNFG KGRGGGFGGN KNFGRGGNFS KRGGFGGSRG KGKYGGKGDD  
61 | YNGFGNDGDN FGGGGSYNDY GNYNNQSSNF DPMGGNFDD RSSGPYDDGG QYFADPRNQG  
121 | GYGGSSSSKS YGSKRRF

(a) **P7KP12Db:**

1 | GSMASASSSQ GGSSGSGNYG GGGGGGYGGN DNYGGGGNYS GSGGYGGSGG GGGYGGSGDG  
61 | YNGYGNDGSN YGGGGSYNDY GNYNNQSSNY GPMKGGNYGG SSSGPYGGGG QYYAKPGNQG  
121 | GYGGSSSSSS YGSGGGY

(b) **M12FP12YM10R:**

1 | GSMASADSSQ RDRDDRGNGF DGRGGGGGGN DNFGRGNGS DRGGGGGSRG DGRYGGDGDR  
61 | YNGGGNDGRN GGGGGSYNDG GNYNNQSSNG DPMKGGNGRD RSSGPYDRGG QYGAKPRNQG  
121 | GYGGSSSSRS YGSDRRG

(c) **M10FP7RP12D:**

1 | GSMASAESSQ REREESGNFG EGRGGGFGGN DNFGRGGNFS ERGGFGGSRG EGGYGGEGDG  
61 | YNGFGNDGSN FGGGGSYNDY GNYNNQSSNF EPMKGGNFGE RSSGPYEGGG QYFAKPRNQG  
121 | GYGGSSSSSS YGSERRF

(d) **P12E:**

1 | GSMASASSSQ RGRSGSGNYG GGRGGGYGGN DNYGRGGNYS GRGGYGGSRG GGGYGGSGDG  
61 | YNGYGNDGSN YGGGGSYNDY GNYNNQSSNY GPMKGGNYGG RSSGGSGGGG QYYAKPRNQG  
121 | GYGGSSSSSS YGSGRRY

(e) **M12FP12Y:**

1 | MDVFMKGLSK AKEGVVAAAE KTKQGVAEAA GKTKEGVLYV GSKTKEGVVH GVATVAEKT  
61 | EQVTNVGGAV VTGVTAVAQK TVEGAGSIAA ATGFVKKDQL GKNEEGAPQE GILEDMPVDP  
121 | DNEAYEMPSE EGYQDYEPEA

(f) **aSyn140:**

1 | SESAWGPAAT IAARQSATGT KTDTPIQKVP QSISVVTAEE MALHQPQSVK EALSYPGVS  
61 | VGTRGASNTY DHLIIRGFAA EGQSQNNYLN GLKLQGNFYN DAVIDPYMLE RAEIMRGPVS  
121 | VLYGKSSPGG LLNMVSKRPT TEPL

(g) **FhuA:**

1 | MSSPGSPGTP GSRSRTPSLP TPPTREPQKV AVVRTPPKSP SSAKSRLQTA PVPMPDLKNV  
61 | KSKIGSTENL KHQPGGGKVQ IVYKPVDSLK VTSKCGSLGN IHHKPGGGQV EVKSEKLDLK  
121 | DRVQSKIGSL DNITHVPGGG NKKIETHKLT FRENAKAKTD HGAEIVY

(h) **K27:**

1 | NAPSTTITTT KQLSRIDSLD NIDHLLDFSS LPPLIDPGFL GQPGPSFSGA RQQHDLKPVL  
61 | HHPTTAPVDN TYLPTQALNF PYHSVHNSGS DFGYGAGSGN NNKGMKLEH SLVSVSQETG  
121 | LSSDVNTTAT PEISSYPMMM NPAMMDGSKS ACDGLDDLIF WEDLYTS

(i) **ANAC046:**

1|MQTAPVPMPD LKNVSKIGS TENLKHQPGG GKVQIVYKPV DLSKVTSKCG SLGNIHHKPG  
61|GGQVEVKSEK LDFKDRVQSK IGSLDNITHV PGGGNKKIET HKLTFRENAK AKTDHGAEIV  
121|YKSPVVGSDT SPRHLSNVSS TGSIDMVDSP QLATLADEV S ASLAKQGL

(a) **K10:**

1|MAEPRQEFEV MEDHAGTYGL GDRKDQGGYT MHQDQEGDTD AGLKAE EAGI GDTPSLEDEA  
61|AGHVTQARMV SKSKDGTGSD DKKAKGADGK TKIATPRGAA PPGQKGQANA TRIPAKTPPA  
121|PKTPSSGEP PKSGDRSGYS SPGSPGTPGS RSRTPSLPTP PTREP KKVAV VRTPPKSPSS  
181|AKSRL

(b) **K25:**

1|MSSPGSPGTP GSRRTPSLP TPPTREP KKV AVVRTPPKSP SSAKSRLQTA PVPMPDLKNV  
61|KSKIGSTENL KHQPGGGKVQ IINKKLDLSN VQSKCGSKDN IKHVPGGGSV QIVYKPDLS  
121|KVTSCGSLG NIHHKPGGGQ VEVKSEK LDF KDRVQSKIGS LDNITHVPGG GNKKIETHKL  
181|TFRENAKAKT DHGAEIVY

(c) **K32:**

1|MSGRNVESHM ERNEKV VVN SGHADVKKQQ QQVEHTEFTH TEVKAPLIHP APPIISTGAA  
61|GLAE EIVGQG FTASAARISG GTAEVHLQPS AAMTEEARRD QERYRQEQES IAKQQUEREME  
121|KKTEAYRKTA EAEAEKIRKE LEKQHARDVE FRKDLIESTI DRQKREVDLE AKMAKRELD R  
181|EGQLAKEALE RSRLATNVEV NFDSAAGHTV SGGTTVSTSD KMEIKRN

(d) **CAHSD:**

1|MAEPRQEFEV MEDHAGTYGL GDRKDQGGYT MHQDQEGDTD AGLKAE EAGI GDTPSLEDEA  
61|AGHVTQARMV SKSKDGTGSD DKKAKGADGK TKIATPRGAA PPGQKGQANA TRIPAKTPPA  
121|PKTPSSGEP PKSGDRSGYS SPGSPGTPGS RSRTPSLPTP PTREP KKVAV VRTPPKSPSS  
181|AKSRLTHKLT FRENAKAKT HGAEIVYKSP VVSGDTSRPH LSNVSSTGSI DMVDSPQLAT  
241|LADEV SASLA KQGL

(e) **K23:**

1|EPPKSGDRSG YSSPGSPGTP GSRRTPSLP TPPTREP KKV AVVRTPPKSP SSAKSRLQTA  
61|PVPMPDLKNV KSKIGSTENL KHQPGGGKVQ IINKKLDLSN VQSKCGSKDN IKHVPGGGSV  
121|QIVYKPDLS KVTSCGSLG NIHHKPGGGQ VEVKSEK LDF KDRVQSKIGS LDNITHVPGG  
181|GNKKIETHKL TFRENAKAKT DHGAEIVYKS PVS GDTSPR HLSNV SSTGS ID MVDSPQLA  
241|TLADEV SASL AKQGL

(f) **tau35:**

1|GPHMQVPRTH RLITLADHIC QIITQDFARN QVPSQASTST FQTSPSALSS TPVRTKTSSR  
61|YSPESQSQT V LHP RP GPRVS PENLVDKSRG SRPGKSPERS HIPSEPYEPI SPPQGPVHE  
121|KQDSMLLSQ RGVDPAEQRS DSRSPGISY LPSFFTKLES TSPMVKSKKQ EIFRKLNSSG  
181|GGDSMAAAQ PGTEIFNLPA VTTSGAVSSR SHSFADPASN LGLEDIIRKA LMGSFDDKVE  
241|DHGVVMSHPV GIMPGSASTS VVTSSEARRD E

(g) **CoRNID:**

|     |            |            |            |            |             |            |
|-----|------------|------------|------------|------------|-------------|------------|
| 1   | MAEPRQEFEV | MEDHAGTYGL | GDRKDQGGYT | MHQDQEGDTD | AGLKAE EAGI | GDTPSLEDEA |
| 61  | AGHVTQARMV | SKSKDGTGSD | DKKAKGADGK | TKIATPRGAA | PPGQKGQANA  | TRIPAKTPPA |
| 121 | PKTPPSSGEP | PKSGDRSGYS | SPGSPGTPGS | RSRTPSLPTP | PTREPKKVAV  | VRTPPKSPSS |
| 181 | AKSRLQTAPV | PMPDLKNVKS | KIGSTENLKH | QPGGGKVQIV | YKPVDSLKVT  | SKCGSLGNIH |
| 241 | HKPGGGQVEV | KSEKLDFKDR | VQSKIGSLDN | ITHVPGGGNK | KIE         |            |

(a) **K44:**

|     |            |            |            |            |             |            |
|-----|------------|------------|------------|------------|-------------|------------|
| 1   | DWNNQSIVKT | GERQHGIHIQ | GSDPGGVRTA | SGTTIKVSGR | QAQGILLENP  | AAELQFRNGS |
| 61  | VTSSGQLSDD | GIEDFLGTVT | VDAGELVADH | ATLANVGDTW | DDDGIALYVA  | GEQAQASIAD |
| 121 | STLQGAGGVQ | IEDGANVTVQ | ESAIVDGGLH | IGALQSLQPR | RLPPSRVVL R | KTNVTAVPAS |
| 181 | GAPAAVSVLG | ASKLTLRGGH | ITGGRAAGVA | AMQGAVVHLQ | RATIRRGRAL  | AGGAVPGGAV |
| 241 | PGGAVPGGFG | PGGFGPVLDG | WYGVDVSGSS | VELAQSIVEA | PELGAAIRVG  | RGARVTVPGG |
| 301 | SLSAPHGNVI | ETGGARRFAP | QAAPLSITLQ | AGAH       |             |            |

(b) **PNtS5:**

|     |            |             |            |            |             |            |
|-----|------------|-------------|------------|------------|-------------|------------|
| 1   | DWNNQSIVKT | GERQHGIHIQ  | GSDPGGVRTA | SGTTIKVSGR | QAQGILLENP  | AAELQFRNGS |
| 61  | VTSSGQLSDD | GIRRF LGTVT | VKAGKLVADH | ATLANVGDTW | DDDGIALYVA  | GEQAQASIAD |
| 121 | STLQGAGGVQ | IERGANVTVQ  | RSAIVDGGLH | IGALQSLQPE | DLPPSRVVL R | DTNVTAVPAS |
| 181 | GAPAAVSVLG | ASELTLDG GH | ITGGRAAGVA | AMQGAVVHLQ | RATIRRGEAL  | AGGAVPGGAV |
| 241 | PGGAVPGGFG | PGGFGPVLDG  | WYGVDVSGSS | VELAQSIVEA | PELGAAIRVG  | RGARVTVPGG |
| 301 | SLSAPHGNVI | ETGGARRFAP  | QAAPLSITLQ | AGAH       |             |            |

(c) **PNt:**

|     |            |             |            |            |             |            |
|-----|------------|-------------|------------|------------|-------------|------------|
| 1   | DWNNQSIVKT | GERQHGIHIQ  | GSDPGGVRTA | SGTTIKVSGR | QAQGILLENP  | AAELQFRNGS |
| 61  | VTSSGQKSDD | GIRRF LGTVT | VLAKKLVADH | ATLANVGDTW | DDDGIALYVA  | GEQAQASIAD |
| 121 | STLQGAGGVQ | IERGANVTVQ  | RSAIVLGGLH | IGALQSLQPE | DDPPSRVVL R | DTNVTAVPAS |
| 181 | GAPAAVSVLG | ASLLTLDG GH | ITGGRAAGVA | AMQGAVVHEQ | RATIRRGEAL  | AGGAVPGGAV |
| 241 | PGGAVPGGFG | PGGFGPVLDG  | WYGVDVSGSS | VELAQSIVEA | PELGAAIRVG  | RGARVTVPGG |
| 301 | SLSAPHGNVI | ETGGARRFAP  | QAAPLSITLQ | AGAH       |             |            |

(d) **PNtS1:**

|     |            |             |            |            |            |            |
|-----|------------|-------------|------------|------------|------------|------------|
| 1   | DWNNQSIVKT | GERQHGIHIQ  | GSDPGGVRTA | SGTTIKVSGR | QAQGILLENP | AAELQFRNGS |
| 61  | VTSSGQLSFV | GITRDLGRDT  | VKAGKLVADH | ATLANVGDTW | DDDGIALYVA | GEQAQASIAD |
| 121 | STLQGAGGVQ | IERGADV RVQ | REAIVDGGLH | NGALQSLQPS | ILPPSTVVLR | DTNVTAVPAS |
| 181 | GAPAAVLVSG | ASGLRLDG GH | IHEGRAAGVA | AMQGAVVTLQ | TATIRRGEAL | AGGAVPGGAV |
| 241 | PGGAVPGGFG | PGGFGPVLDG  | WYGVDVSGSS | VELAQSIVEA | PELGAAIRVG | RGARVTVPGG |
| 301 | SLSAPHGNVI | ETGGARRFAP  | QAAPLSITLQ | AGAH       |            |            |

(e) **PNtS4:**

|     |            |            |            |            |            |            |
|-----|------------|------------|------------|------------|------------|------------|
| 1   | DWNNQSIVKT | GERQHGIHIQ | GSDPGGVRTA | SGTTIKVSGR | QAQGILLENP | AAELQFRNGS |
| 61  | VTSSGQLSDR | GIDRFLGTVT | VEAGKLVADH | ATLANVGDTW | DKDGIALYVA | GRQQAQSIAD |
| 121 | STLQGAGGVQ | IREGANVTVQ | RSAIVDGGLH | IGALQSLQPE | RLPPSDVVL  | DTNVTAVPAS |
| 181 | GAPAAVSVLG | ASRLTLDGGH | ITGGDAAGVA | AMQGAVVHLQ | RATIERGEAL | AGGAVPGGAV |
| 241 | PGGAVPGGFG | PGGFGPVL   | WYGVDVSGSS | VELAQSIVEA | PELGAAIRVG | RGARVTVPGG |
| 301 | SLSAPHGNVI | ETGGARRFAP | QAAPLSITLQ | AGAH       |            |            |

(a) **PNtS6:**

|     |            |            |            |            |            |            |
|-----|------------|------------|------------|------------|------------|------------|
| 1   | SKQQRIKMLI | LPPVPVPKIK | GIDPDLKEG  | KLEEVNTILA | IHDSYKPEFH | SDDSWVEFIE |
| 61  | LDIDEPDEKT | EESDTRLLS  | SDHEKSHSNL | GVKDGDSGRT | SCCEPDILET | DFNANDIHEG |
| 121 | TSEVAQPQRL | KGEADLLCLD | QKNQNNSPYH | DACPATQQPS | VIQAEKNKPQ | PLPTEGAEST |
| 181 | HQAAHIQLSN | PSSLSNIDFY | AQVSDITPAG | SVVLSPGQKN | KAGMSQCDMH | PEMVSLCQEN |
| 241 | FLMDNAYFCE | ADAKKCIPIV | PHIKVESHIQ | PSLNQEDIYI | TTESLTAAAG | RPGTGEHVP  |
| 301 | SEMPVPDYTS | IHIVQSPQGL | ILNATALPLP | DKEFLSSCGY | VSTDQLNKIM | P          |

(b) **GHRICD:**

|     |            |            |            |            |            |            |
|-----|------------|------------|------------|------------|------------|------------|
| 1   | MAEPRQEFEV | MEDHAGTYGL | GDRKDQGGYT | MHQDQEGDTD | AGLKESPLQT | PTEDGSEEPG |
| 61  | SETSDAKSTP | TAEDVTAPLV | DEGAPGKQAA | AQPHTEIPEG | TTAEEAGIGD | TPSLEDEAAG |
| 121 | HVTQARMVSK | SKDGTGSDDK | KAKGADGKTK | IATPRGAAPP | GQKGQANATR | IPAKTPPAPK |
| 181 | TPSSSGEPPK | SGDRSGYSSP | GSPGTPGSR  | RTPSLPTPPT | REPKKVAVVR | TPPKSPSSAK |
| 241 | SRLQTAPVPM | PDLKNVSKSI | GSTENLKHQP | GGGKVQIVYK | PVDLSKVTSK | CGSLGNIHHK |
| 301 | PGGGQVEVKS | EKLDFKDRVQ | SKIGSLDNIT | HVPGGGNKKI | ETHKLTFREN | AKAKTDHGAE |
| 361 | IVYKSPVVS  | DTSPRHLSNV | SSTGSIDMVD | SPQLATLADE | VSASLAKQGL |            |

(c) **ht2N3R:**

|     |            |            |            |            |            |            |
|-----|------------|------------|------------|------------|------------|------------|
| 1   | MAEPRQEFEV | MEDHAGTYGL | GDRKDQGGYT | MHQDQEGDTD | AGLKESPLQT | PTEDGSEEPG |
| 61  | SETSDAKSTP | TAEDVTAPLV | DEGAPGKQAA | AQPHTEIPEG | TTAEEAGIGD | TPSLEDEAAG |
| 121 | HVTQARMVSK | SKDGTGSDDK | KAKGADGKTK | IATPRGAAPP | GQKGQANATR | IPAKTPPAPK |
| 181 | TPSSSGEPPK | SGDRSGYSSP | GSPGTPGSR  | RTPSLPTPPT | REPKKVAVVR | TPPKSPSSAK |
| 241 | SRLQTAPVPM | PDLKNVSKSI | GSTENLKHQP | GGGKVQIINK | KLDLSNVQSK | CGSKDNIHKV |
| 301 | PGGGSVQIVY | KPVDLSKVTS | KCGSLGNIHH | KPGGGQVEVK | SEKLDFKDRV | QSKIGSLDNI |
| 361 | THVPGGGNKK | IETHKLTFRE | NAKAKTDHGA | EIVYKSPVVS | GDTSPRHLSN | VSSTGSIDMV |
| 421 | DSPQLATLAD | EVSASLAKQG | L          |            |            |            |

(d) **ht2N4R:**

### III. SEQUENCE INFORMATION

| Name    | #Particles | $f_+^3$ | $f_-^3$ | $f_{cr}^3$ | $ncpr^3$ | $\kappa^3$ | $\delta^3$ | SCD <sup>4</sup> | nSCD <sup>5</sup> |
|---------|------------|---------|---------|------------|----------|------------|------------|------------------|-------------------|
| Hst5    | 24         | 0.58    | 0.083   | 0.67       | 0.50     | 0.30       | 0.37       | 0.87             | 0.25              |
| Hst52   | 48         | 0.58    | 0.083   | 0.67       | 0.50     | 0.30       | 0.37       | 4.3              | 0.13              |
| p532070 | 62         | 0.13    | 0.21    | 0.34       | 0.081    | 0.30       | 0.019      | 2.7              | 0.26              |
| ACTR    | 71         | 0.085   | 0.18    | 0.27       | 0.099    | 0.15       | 0.036      | 1.3              | 0.12              |
| DSS1    | 71         | 0.070   | 0.32    | 0.39       | 0.25     | 0.39       | 0.16       | 6.9              | 0.31              |
| Ash1    | 81         | 0.22    | 0.012   | 0.23       | 0.21     | 0.19       | 0.19       | 6.3              | 0.15              |
| CTD2    | 83         | 0       | 0       | 0          | 0        | -          | -          | 0                | -                 |
| Sic1    | 92         | 0.12    | 0       | 0.12       | 0.12     | 0.21       | 0.12       | 3.4              | 0.076             |
| SH4UD   | 95         | 0.15    | 0.074   | 0.22       | 0.074    | 0.17       | 0.025      | 0.11             | 0.046             |
| ColNT   | 98         | 0.18    | 0.051   | 0.23       | 0.13     | 0.24       | 0.075      | -0.080           | 0.056             |
| p27Cv15 | 107        | 0.16    | 0.13    | 0.29       | 0.028    | 0.15       | 0.0027     | -0.75            | 0.050             |
| p27Cv31 | 107        | 0.16    | 0.13    | 0.29       | 0.028    | 0.28       | 0.0027     | -0.94            | 0.063             |
| p27Cv44 | 107        | 0.16    | 0.13    | 0.29       | 0.028    | 0.40       | 0.0027     | -1.5             | 0.10              |
| p27Cv56 | 107        | 0.16    | 0.13    | 0.29       | 0.028    | 0.54       | 0.0027     | -3.9             | 0.26              |
| p27Cv78 | 107        | 0.16    | 0.13    | 0.29       | 0.028    | 0.77       | 0.0027     | -7.6             | 0.51              |
| p27Cv14 | 107        | 0.16    | 0.13    | 0.29       | 0.028    | 0.15       | 0.0027     | -0.61            | 0.040             |
| p15PAF  | 111        | 0.20    | 0.11    | 0.31       | 0.090    | 0.19       | 0.026      | 0.67             | 0.084             |
| PTMA    | 111        | 0.090   | 0.48    | 0.57       | 0.39     | 0.42       | 0.26       | 39               | 0.23              |
| NHE6cmd | 116        | 0.086   | 0.17    | 0.26       | 0.086    | 0.22       | 0.029      | 2.6              | 0.095             |
| hNL3cyt | 119        | 0.14    | 0.10    | 0.24       | 0.042    | 0.18       | 0.0072     | -0.87            | 0.091             |
| RNaseA  | 124        | 0.15    | 0.081   | 0.23       | 0.065    | 0.12       | 0.018      | -0.018           | 0.037             |
| A1S150  | 131        | 0.092   | 0.023   | 0.11       | 0.069    | 0.20       | 0.041      | 1.8              | 0.054             |
| M4D     | 137        | 0.088   | 0       | 0.088      | 0.088    | 0.19       | 0.088      | 3.4              | 0.069             |
| M8FP4Y  | 137        | 0.088   | 0.029   | 0.12       | 0.058    | 0.22       | 0.029      | 1.3              | 0.054             |
| M9FP3Y  | 137        | 0.088   | 0.029   | 0.12       | 0.058    | 0.22       | 0.029      | 1.3              | 0.054             |
| M10R    | 137        | 0.015   | 0.029   | 0.044      | 0.015    | 0.36       | 0.0049     | -0.14            | 0.31              |
| M6R     | 137        | 0.044   | 0.029   | 0.073      | 0.015    | 0.26       | 0.0029     | -0.088           | 0.079             |
| P2R     | 137        | 0.10    | 0.029   | 0.13       | 0.073    | 0.17       | 0.041      | 2.3              | 0.037             |
| P7R     | 137        | 0.14    | 0.029   | 0.17       | 0.11     | 0.15       | 0.071      | 5.2              | 0.055             |
| P8D     | 137        | 0.088   | 0.088   | 0.18       | 0        | 0.11       | 0          | -0.37            | 0.037             |
| P12D    | 137        | 0.088   | 0.12    | 0.20       | 0.029    | 0.12       | 0.0042     | -0.32            | 0.048             |
| M9FP6Y  | 137        | 0.088   | 0.029   | 0.12       | 0.058    | 0.22       | 0.029      | 1.3              | 0.054             |
| M6RP6K  | 137        | 0.088   | 0.029   | 0.12       | 0.058    | 0.22       | 0.029      | 1.3              | 0.054             |

| Name         | #Particles | $f_+^3$ | $f_-^3$ | fcr <sup>3</sup> | ncpr <sup>3</sup> | $\kappa^3$ | $\delta^3$ | SCD <sup>4</sup> | nSCD <sup>5</sup> |
|--------------|------------|---------|---------|------------------|-------------------|------------|------------|------------------|-------------------|
| P4D          | 137        | 0.088   | 0.058   | 0.15             | 0.029             | 0.15       | 0.0058     | 0.15             | 0.027             |
| M10RP10K     | 137        | 0.088   | 0.029   | 0.12             | 0.058             | 0.22       | 0.029      | 1.3              | 0.054             |
| M3RP3K       | 137        | 0.088   | 0.029   | 0.12             | 0.058             | 0.22       | 0.029      | 1.3              | 0.054             |
| P7FM7Y       | 137        | 0.088   | 0.029   | 0.12             | 0.058             | 0.22       | 0.029      | 1.3              | 0.054             |
| P7KP12D      | 137        | 0.14    | 0.12    | 0.26             | 0.022             | 0.076      | 0.0019     | -0.42            | 0.027             |
| A1           | 137        | 0.088   | 0.029   | 0.12             | 0.058             | 0.22       | 0.029      | 1.3              | 0.054             |
| P7KP12Db     | 137        | 0.14    | 0.12    | 0.26             | 0.022             | 0.24       | 0.0019     | -1.2             | 0.067             |
| M12FP12YM10R | 137        | 0.015   | 0.029   | 0.044            | 0.015             | 0.36       | 0.0049     | -0.14            | 0.31              |
| M10FP7RP12D  | 137        | 0.14    | 0.12    | 0.26             | 0.022             | 0.076      | 0.0019     | -0.42            | 0.027             |
| P12E         | 137        | 0.088   | 0.12    | 0.20             | 0.029             | 0.12       | 0.0042     | -0.32            | 0.048             |
| M12FP12Y     | 137        | 0.088   | 0.029   | 0.12             | 0.058             | 0.22       | 0.029      | 1.3              | 0.054             |
| aSyn140      | 140        | 0.11    | 0.17    | 0.29             | 0.057             | 0.17       | 0.011      | -1.3             | 0.14              |
| FhuA         | 144        | 0.10    | 0.083   | 0.19             | 0.021             | 0.17       | 0.0023     | -0.24            | 0.023             |
| K27          | 167        | 0.21    | 0.078   | 0.29             | 0.13              | 0.13       | 0.060      | 4.6              | 0.054             |
| ANAC046      | 167        | 0.084   | 0.11    | 0.19             | 0.024             | 0.20       | 0.0030     | 1.8              | 0.055             |
| K10          | 168        | 0.18    | 0.10    | 0.28             | 0.077             | 0.16       | 0.021      | -0.21            | 0.043             |
| K25          | 185        | 0.17    | 0.13    | 0.30             | 0.038             | 0.17       | 0.0048     | -4.8             | 0.14              |
| K32          | 198        | 0.21    | 0.076   | 0.28             | 0.13              | 0.12       | 0.061      | 6.2              | 0.051             |
| CAHSD        | 227        | 0.20    | 0.19    | 0.38             | 0.013             | 0.072      | 0.00046    | -0.10            | 0.0043            |
| K23          | 254        | 0.16    | 0.13    | 0.29             | 0.035             | 0.18       | 0.0044     | -3.8             | 0.074             |
| tau35        | 255        | 0.18    | 0.086   | 0.27             | 0.098             | 0.14       | 0.036      | 2.9              | 0.060             |
| CoRNID       | 271        | 0.14    | 0.10    | 0.24             | 0.037             | 0.16       | 0.0056     | -1.1             | 0.027             |
| K44          | 283        | 0.18    | 0.12    | 0.30             | 0.064             | 0.16       | 0.014      | -3.2             | 0.082             |
| PNtS5        | 334        | 0.093   | 0.084   | 0.18             | 0.0090            | 0.27       | 0.00046    | -2.5             | 0.095             |
| PNt          | 334        | 0.093   | 0.084   | 0.18             | 0.0090            | 0.21       | 0.00046    | -0.38            | 0.023             |
| PNtS1        | 334        | 0.093   | 0.084   | 0.18             | 0.0090            | 0.20       | 0.00046    | -0.36            | 0.022             |
| PNtS4        | 334        | 0.093   | 0.084   | 0.18             | 0.0090            | 0.16       | 0.00046    | -0.33            | 0.021             |
| PNtS6        | 334        | 0.093   | 0.084   | 0.18             | 0.0090            | 0.14       | 0.00046    | -0.11            | 0.014             |
| GHRICD       | 351        | 0.11    | 0.16    | 0.27             | 0.048             | 0.16       | 0.0087     | 10               | 0.054             |
| ht2N3R       | 410        | 0.16    | 0.13    | 0.29             | 0.024             | 0.19       | 0.0021     | -7.6             | 0.072             |
| ht2N4R       | 441        | 0.16    | 0.13    | 0.29             | 0.032             | 0.18       | 0.0035     | -8.1             | 0.070             |

Table S1: Characteristic features of charge patterning of the different protein sequences.

#### IV. ADDITIONAL SIMULATION RESULTS

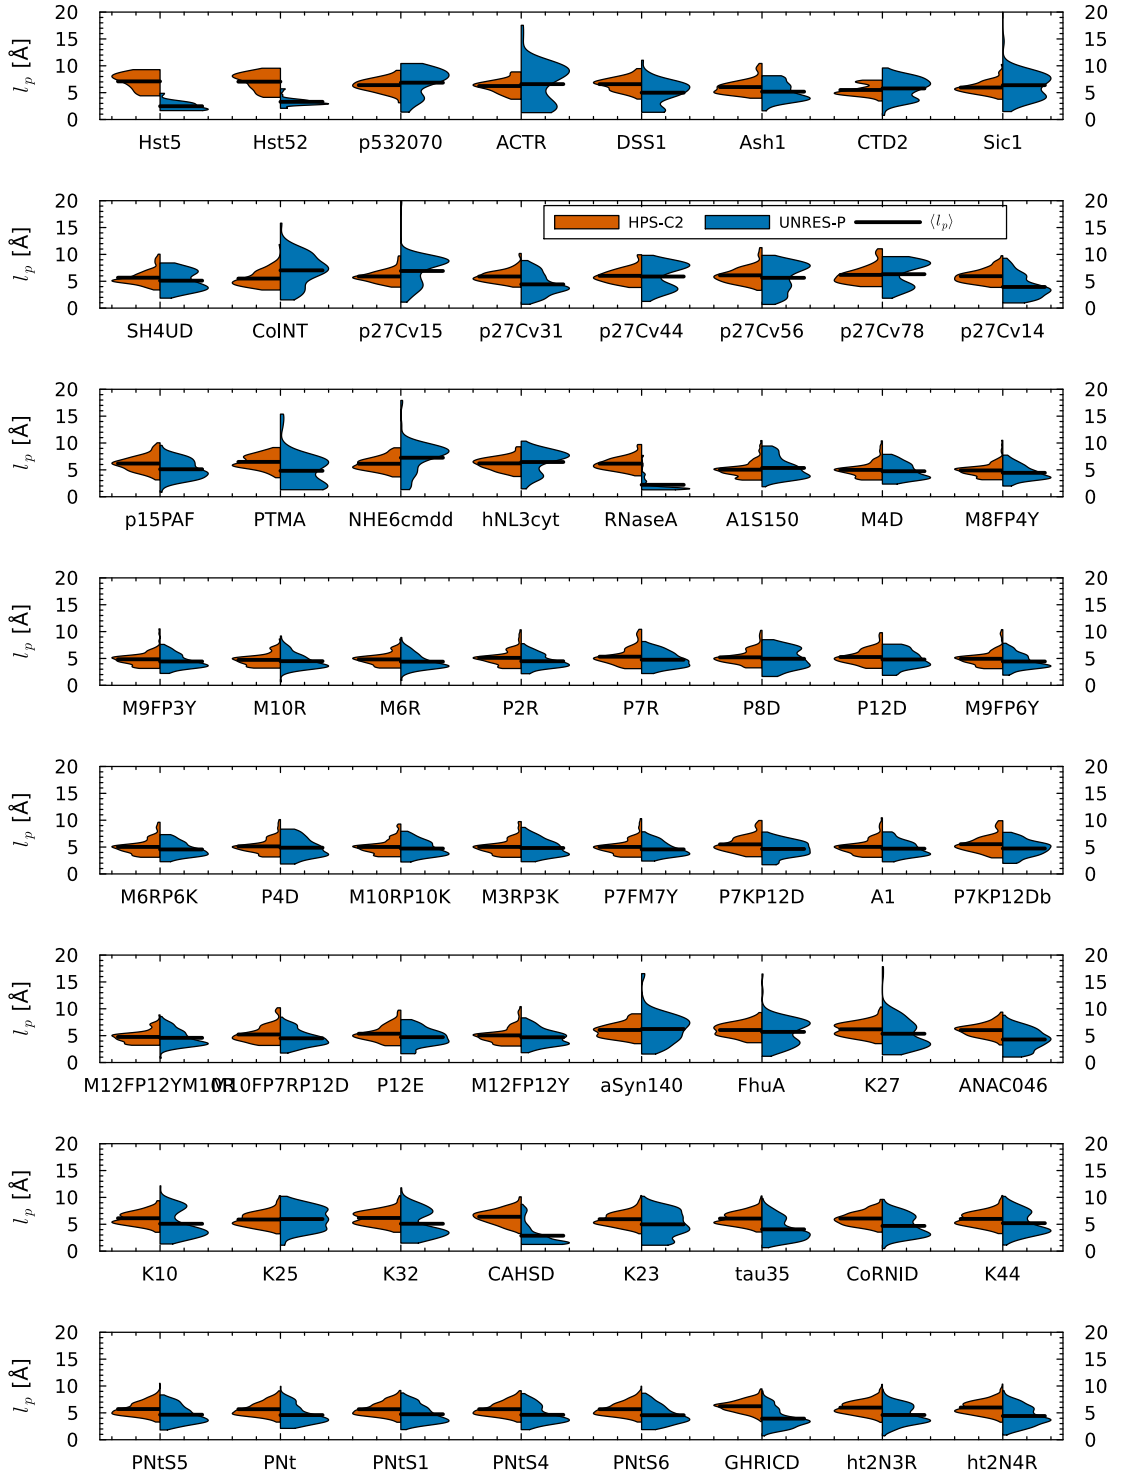

Figure S1: Distribution of the local persistence lengths for IDPs simulated with the HPS-C2 and UNRES-P models. Black lines indicate the arithmetic mean of  $\ell_{p,i}$ .

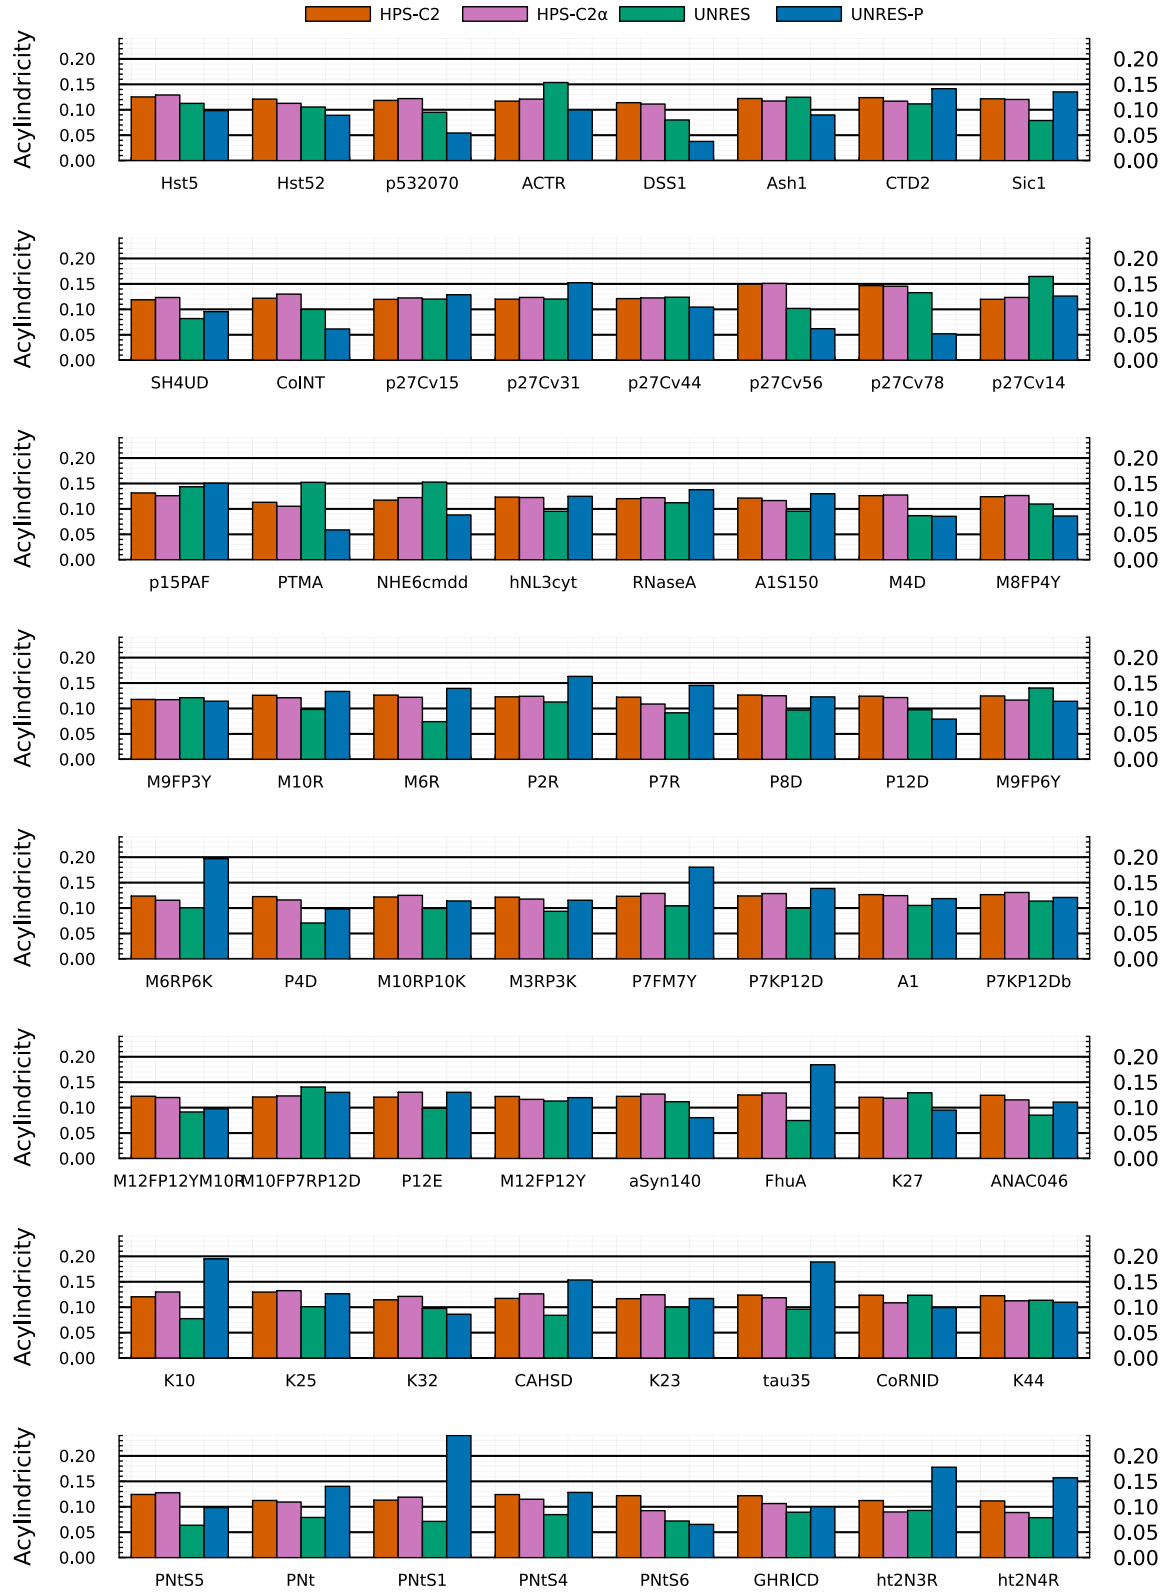

Figure S2: Acylindricity for IDPs simulated using the HPS-C2, HPS-C2 $\alpha$ , UNRES and UNRES-P models.

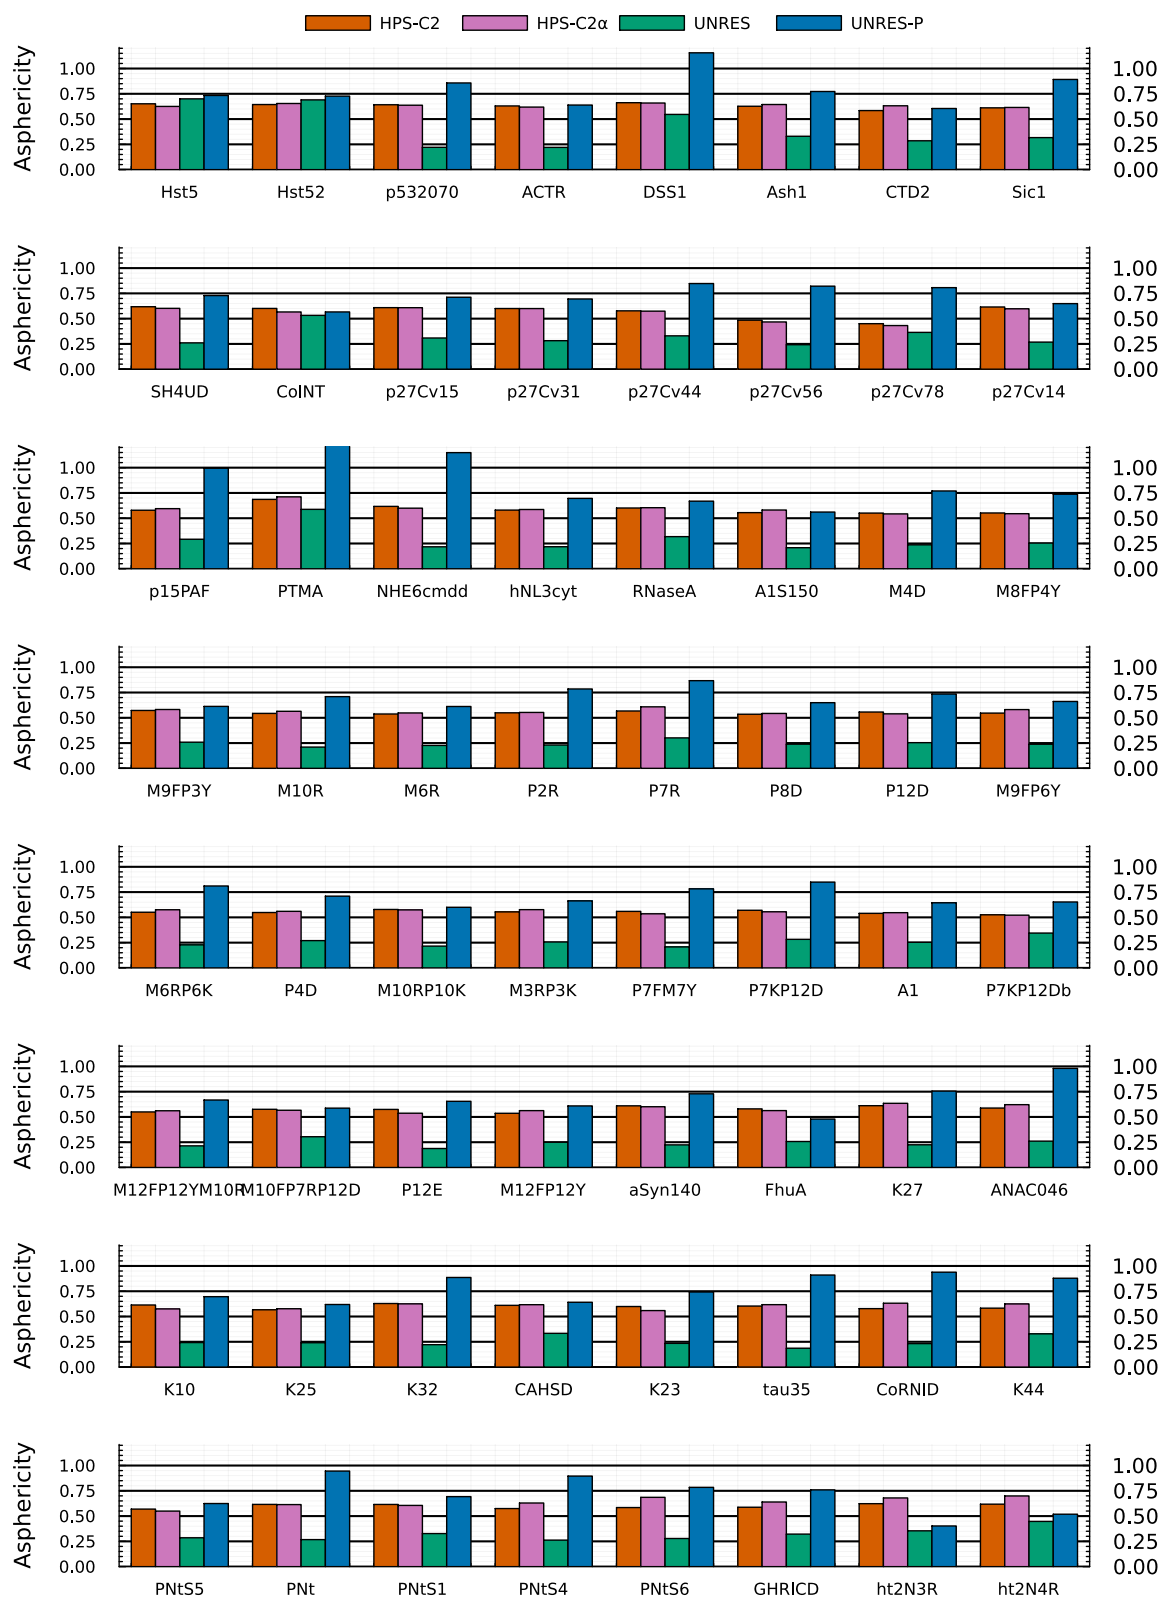

Figure S3: Asphericity for IDPs simulated using the HPS-C2, HPS-C2 $\alpha$ , UNRES and UNRES-P models.

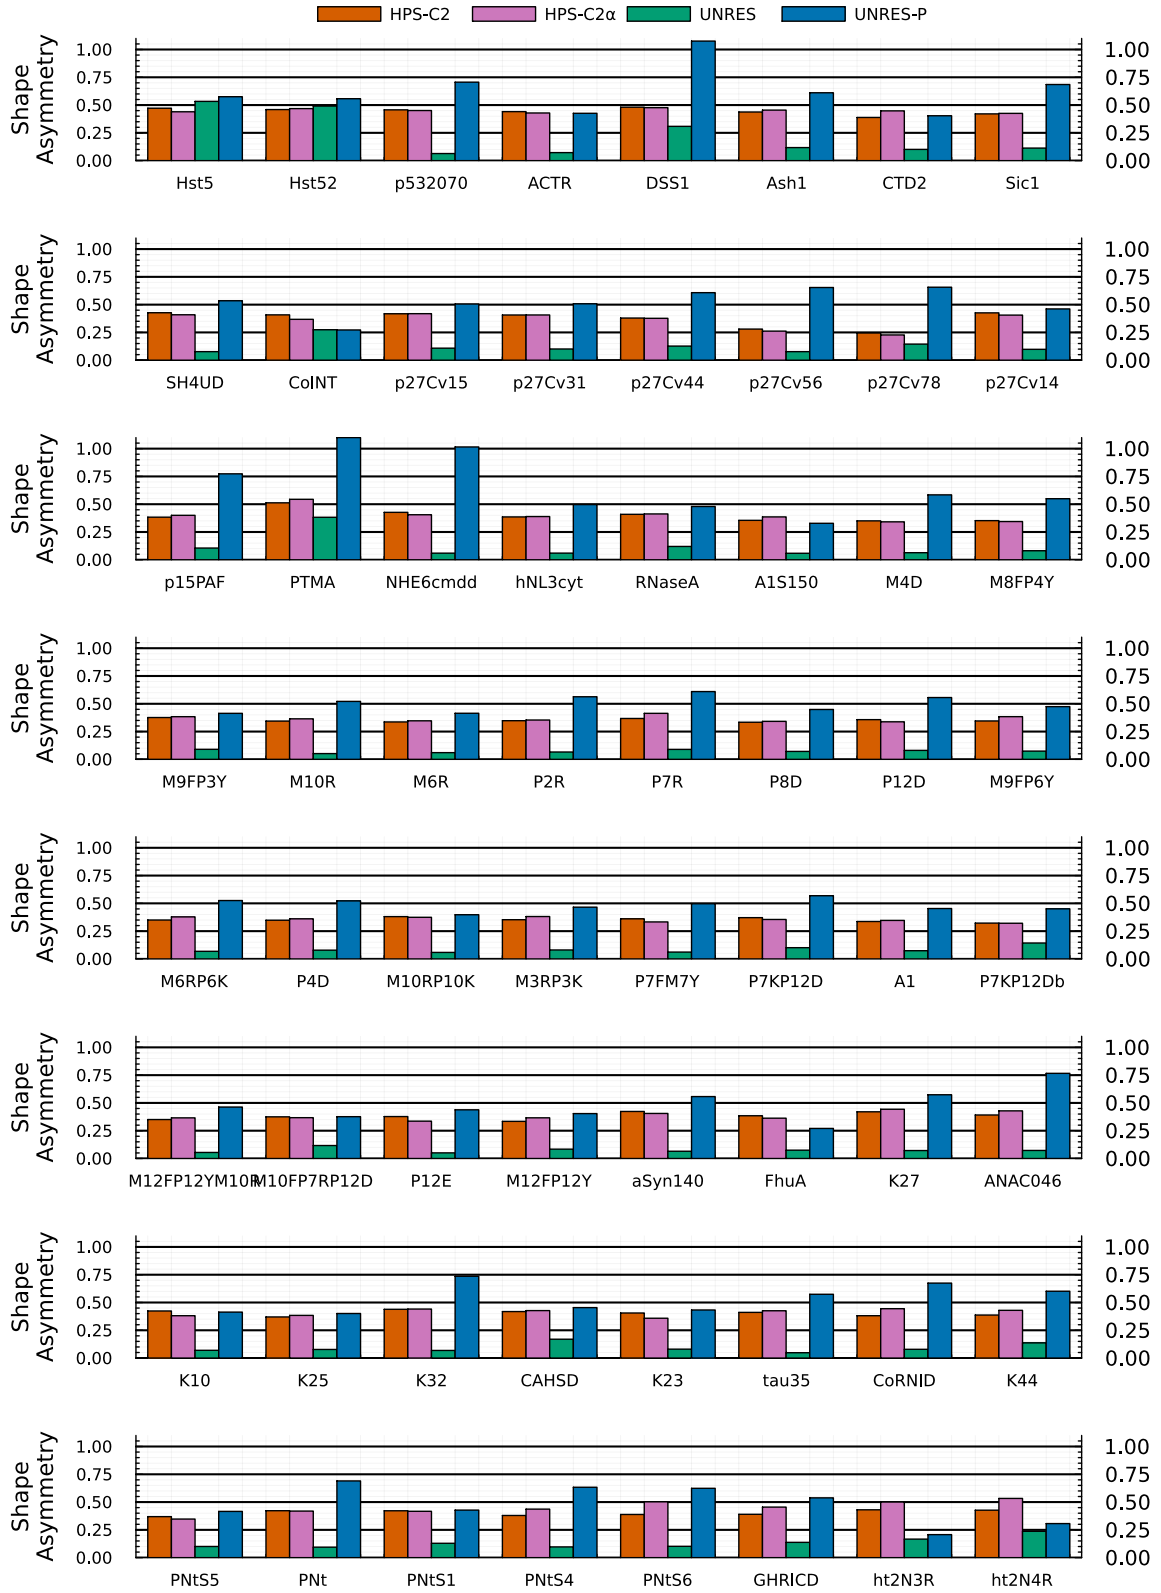

Figure S4: Relative shape anisotropy for IDPs simulated using the HPS-C2, HPS-C2 $\alpha$ , UNRES and UNRES-P models.

## REFERENCES

- <sup>1</sup>M. Doi, S. F. Edwards, and S. F. Edwards, *The Theory of Polymer Dynamics* (Clarendon Press, 1988).
- <sup>2</sup>D. S. Broca, Int. J. Math. Educ. Sci. Technol. **35**, 917 (2004).
- <sup>3</sup>R. K. Das and R. V. Pappu, Proc. Natl. Acad. Sci. U. S. A. **110**, 13392 (2013).
- <sup>4</sup>L. Sawle and K. Ghosh, J. Chem. Physics. **143**, 085101 (2015).
- <sup>5</sup>D. S. Devarajan, S. Rekhi, A. Nikoubashman, Y. C. Kim, M. P. Howard, and J. Mittal, Macromolecules **55**, 8987 (2022).
